# Supplementary material for: Rethinking the Unsupervised Paradigm in Time Series Anomaly Detection: An Empirical Study and Minimalist Baseline
Source: arXiv:2511.16145 source file (2026-11-03)
Supplement: Supplementary file 1 [file supp.tex]

% supp.tex
% 检查是否被主文件包含：若未被包含，则加载完整文档结构（期刊独立版）
\ifx\includedfrommain\undefined
  % 独立编译时的文档设置（与主文件保持一致的文档类和宏包）
    \documentclass[lettersize,journal]{IEEEtran}
    \usepackage{xr-hyper}
    \usepackage{hyperref}
    \usepackage{amsmath,amsfonts}
    \usepackage{algorithmic}
    \usepackage{algorithm}
    \usepackage{array}
    \usepackage[caption=false,font=normalsize,labelfont=sf,textfont=sf]{subfig}
    \usepackage{textcomp}
    \usepackage{url}
    \usepackage{verbatim}
    \usepackage{graphicx}

    \usepackage{pifont}
    
    \usepackage{hyperref}
    \usepackage{url}
    
    \usepackage{booktabs}       % professional-quality tables
    \usepackage{nicefrac}       % compact symbols for 1/2, etc.
    \usepackage{microtype}      % microtypography
    \usepackage{xcolor}         % colors
    \usepackage{graphicx}
    \usepackage[normalem]{ulem} 
    \usepackage{multirow}
    \usepackage{multicol}
    % \usepackage{subcaption}
    % \usepackage{wrapfig}
% 4. 颜色支持（适配 \textcolor{gray}{...} 灰色注释）

\usepackage{color}         % colors
\usepackage{colortbl}
    
    \usepackage[scr=boondox,cal=esstix]{mathalpha}
    \usepackage{float}                  % 图片浮动位置
    \usepackage{overpic}                % 叭啦叭啦，与图片排版相关\
    \usepackage{listings}
    \usepackage[numbers]{natbib}
    
    % % copy labels
    % \usepackage{xr}
    % \externaldocument{output}
    
    % % copy citations
    % \usepackage{xcite}
    % \externalcitedocument{output}

    \lstset{
    language=Python,  % 设置语言为Python
    basicstyle=\ttfamily,  % 设置基本字体样式
    tabsize=4,  % 设置制表符宽度
    numbers=left,  % 行号显示在左边
    numberstyle=\tiny\color{gray},  % 行号样式
    breaklines=true,  % 自动换行
    frame=single,  % 代码块框架
    stringstyle  = \color{purple},
    keywordstyle = \color{blue!60!black}\bfseries,
    commentstyle = \color{green!40!black}\scshape,
    xleftmargin      = 20pt,
    xrightmargin     = 0pt,
    aboveskip=5pt,
    belowskip=-2.2pt,
    frame            = tb,
    framesep         = \fboxsep,
    framexleftmargin = 20pt,
    breaklines=true,
}
  \newcommand{\stand}{\texttt{STAND}}
  \externaldocument{main} % 关联主文件的引用（独立编译时用）
  \begin{document}
\fi

% 定义默认颜色为蓝色的命令
% \newcommand{\rv}[1]{\textcolor{blue}{#1}}

\renewcommand{\thetable}{A\arabic{table}}
\renewcommand{\thefigure}{A\arabic{figure}}
\renewcommand{\thealgorithm}{A\arabic{algorithm}}

\hyphenation{op-tical net-works semi-conduc-tor IEEE-Xplore}
% updated with editorial comments 8/9/2021

\setcounter{section}{0}
\renewcommand{\thesection}{\Alph{section}}

% \newpage
% \appendix

% \title{Labels Matter More Than Models: Quantifying the Benefit of Supervised Time Series Anomaly Detection}
% \title{Labels Matter More Than Models: Rethinking the Unsupervised Paradigm in Time Series Anomaly Detection}

\section*{Appendix}

This is the appendix of \textit{Labels Matter More Than Models: Rethinking the Unsupervised Paradigm in Time Series Anomaly Detection}.

% \section{无监督方法的对比结果}\label{app:utad_comparison}
% 表\ref{tab:comparison_utad}展示了所有无监督方法（UTAD-I和UTAD-II两类）的结果.
\section{Full Results of Unsupervised Methods}\label{app:utad_comparison}
Table \ref{tab:comparison_utad} presents the complete results for all unsupervised methods (including both UTAD-I and UTAD-II categories).

\begin{table*}[htbp]
  \centering
  % \caption{所有无监督方法在五个数据集六种指标上的表现对比。\textbf{加粗}表示最佳表现，\uline{下划线}表示次佳表现。灰色高亮的方法是UTAD-I，绿色高亮的方法是UTAD-II。}
  \caption{Performance comparison of all unsupervised methods across five datasets and six metrics. \textbf{Bold} indicates the best performance, and \uline{underlining} indicates the second-best performance. Methods highlighted in gray are UTAD-I, and methods highlighted in green are UTAD-II.}
  \resizebox{\linewidth}{!}{
    \begin{tabular}{c|cccccc|cccccc|cccccc}
    \toprule
    \textbf{Dataset} & \multicolumn{6}{c|}{\textbf{PSM}}             & \multicolumn{6}{c|}{\textbf{SWaT}}            & \multicolumn{6}{c}{\textbf{WADI}} \\
    \midrule
    \textbf{Metric} & \textbf{CCE} & \textbf{F1} & \textbf{Aff-F1} & \textbf{UAff-F1} & \textbf{AUC-ROC} & \textbf{VUS-PR} & \textbf{CCE} & \textbf{F1} & \textbf{Aff-F1} & \textbf{UAff-F1} & \textbf{AUC-ROC} & \textbf{VUS-PR} & \textbf{CCE} & \textbf{F1} & \textbf{Aff-F1} & \textbf{UAff-F1} & \textbf{AUC-ROC} & \textbf{VUS-PR} \\
    \midrule
    \rowcolor[rgb]{ .949,  .949,  .949} Random & -0.83  & 8.51  & 67.99  & 5.53  & 50.10  & 32.99  & -0.48  & 7.07  & 68.96  & -3.13  & 49.96  & 12.77  & -0.07  & 4.90  & 69.16  & -6.51  & 49.80  & 8.47  \\
    \rowcolor[rgb]{ .949,  .949,  .949} IForest & -5.40  & 3.75  & 49.60  & -1.69  & 46.76  & 29.96  & -2.02  & 6.02  & 62.11  & -9.86  & 32.74  & 10.37  & 7.83  & 10.99  & 61.99  & -11.06  & 74.70  & 17.17  \\
    \rowcolor[rgb]{ .949,  .949,  .949} LOF   & 0.39  & 10.09  & 73.93  & 23.52  & 51.71  & 35.40  & 0.06  & 8.08  & 72.90  & 17.03  & 50.60  & 13.68  & 0.93  & 9.32  & 74.42  & 28.97  & 55.18  & 11.16  \\
    \rowcolor[rgb]{ .949,  .949,  .949} PCA   & \uline{6.56 } & 18.77  & 57.93  & 52.38  & \textbf{74.13 } & \textbf{55.01 } & 4.52  & 48.84  & 66.17  & 30.80  & \textbf{89.73 } & 61.73  & \uline{14.39 } & \textbf{39.07 } & \textbf{81.74 } & \textbf{58.92 } & \uline{81.07 } & \uline{37.04 } \\
    \rowcolor[rgb]{ .949,  .949,  .949} HBOS  & -3.44  & 8.52  & 44.79  & -18.88  & 49.90  & 33.23  & 9.65  & 10.38  & 71.49  & 24.54  & 75.08  & 26.34  & 9.44  & 9.86  & 67.40  & 6.38  & 73.97  & 18.50  \\
    \rowcolor[rgb]{ .949,  .949,  .949} KNN   & -1.78  & 9.08  & 70.11  & 31.22  & 37.39  & 29.49  & -1.95  & 4.17  & 70.06  & 10.90  & 14.49  & 7.78  & -0.37  & 5.23  & 68.68  & -6.21  & 51.76  & 10.31  \\
    \rowcolor[rgb]{ .949,  .949,  .949} KMeans & 0.12  & 7.85  & 60.05  & 44.55  & 38.64  & 30.14  & 4.79  & 19.49  & \textbf{78.12 } & \textbf{46.24 } & 33.06  & 18.18  & 6.46  & 12.72  & 66.56  & 28.87  & 64.70  & 13.79  \\
    \midrule
    \midrule
    \rowcolor[rgb]{ .886,  .937,  .855} OCSVM & 2.84  & 17.03  & 43.42  & 30.49  & 52.63  & 38.46  & 10.10  & 4.77  & 39.06  & 21.13  & 77.36  & 24.78  & 13.37  & 32.12  & 70.40  & 47.82  & \textbf{81.78 } & 32.00  \\
    \rowcolor[rgb]{ .886,  .937,  .855} AE    & \textbf{\uline{7.78 }} & 5.19  & 56.50  & 51.07  & 56.50  & 34.90  & 16.25  & 17.87  & 74.95  & 40.34  & 84.69  & 45.08  & \textbf{15.04 } & 27.00  & 74.26  & 42.28  & 64.38  & 16.65  \\
    \rowcolor[rgb]{ .886,  .937,  .855} CNN   & 0.57  & \uline{26.33 } & 69.16  & \uline{60.48 } & 61.26  & \uline{52.52 } & 29.04  & \textbf{58.34 } & 5.46  & 5.46  & 86.77  & 60.84  & 2.39  & 24.20  & 78.57  & 43.04  & 66.08  & 24.00  \\
    \rowcolor[rgb]{ .886,  .937,  .855} LSTM  & 0.60  & \textbf{26.86 } & 66.48  & 57.44  & 63.88  & 51.85  & 29.54  & \uline{58.32 } & 5.41  & 5.41  & 86.63  & \textbf{68.63 } & 2.47  & 23.98  & \uline{78.70 } & 43.07  & 70.80  & 25.67  \\
    \rowcolor[rgb]{ .886,  .937,  .855} TranAD & 0.23  & 20.09  & 63.50  & 58.40  & 60.54  & 46.85  & 29.78  & \textbf{58.34 } & 5.34  & 5.34  & 88.47  & \uline{63.50 } & 2.60  & 23.23  & 77.80  & 40.01  & 72.76  & 30.27  \\
    \rowcolor[rgb]{ .886,  .937,  .855} USAD  & 1.49  & 21.39  & 46.14  & 44.90  & 61.53  & 46.62  & \uline{29.79 } & \textbf{58.34 } & 5.33  & 5.33  & 88.71  & 63.04  & 8.36  & 23.01  & 77.83  & 39.86  & 73.60  & 28.02  \\
    \rowcolor[rgb]{ .886,  .937,  .855} Omni  & 3.93  & 21.78  & 23.44  & 23.04  & \uline{64.11 } & 44.55  & \textbf{29.80 } & \textbf{58.34 } & 5.31  & 5.31  & \uline{88.85 } & 59.30  & 10.84  & \uline{39.02 } & 72.07  & \uline{52.59 } & 79.13  & \textbf{38.82 } \\
    \rowcolor[rgb]{ .886,  .937,  .855} A.T.  & 1.02  & 18.20  & 48.73  & 42.56  & 59.13  & 43.46  & 29.31  & 58.34  & 5.35  & 5.35  & 74.39  & 47.13  & 3.88  & 28.02  & 74.06  & 22.00  & 61.97  & 20.27  \\
    \rowcolor[rgb]{ .886,  .937,  .855} TimesNet & 0.01  & 15.34  & 73.81  & 35.76  & 57.19  & 46.33  & 0.12  & 8.77  & 74.09  & 30.50  & 30.16  & 11.71  & 0.59  & 16.76  & 73.85  & 18.57  & 70.07  & 20.66  \\
    \rowcolor[rgb]{ .886,  .937,  .855} M2N2  & -0.07  & 15.26  & \uline{79.11 } & 47.11  & 63.35  & 48.17  & 0.01  & 23.99  & \uline{75.65 } & \uline{42.15 } & 81.15  & 33.29  & 1.69  & 20.75  & 74.89  & 22.97  & 64.38  & 22.25  \\
    \rowcolor[rgb]{ .886,  .937,  .855} LFTSAD & -0.32  & 9.27  & 63.57  & 16.99  & 44.32  & 31.62  & 0.81  & 19.79  & 65.12  & 3.58  & 66.36  & 24.21  & 0.28  & 9.54  & 53.74  & -27.72  & 48.41  & 11.49  \\
    \rowcolor[rgb]{ .886,  .937,  .855} CATCH & 0.62  & 16.85  & \textbf{84.85 } & \textbf{62.92 } & 60.65  & 51.99  & 0.02  & 9.33  & 73.41  & 23.84  & 29.78  & 11.87  & 0.26  & 13.64  & 74.92  & 31.67  & 69.76  & 21.18  \\
    \midrule
    \textbf{Dataset} & \multicolumn{6}{c|}{\textbf{Swan}}            & \multicolumn{6}{c|}{\textbf{Water}}           & \multicolumn{6}{c}{\textbf{Average}} \\
    \midrule
    \textbf{Metric} & \textbf{CCE} & \textbf{F1} & \textbf{Aff-F1} & \textbf{UAff-F1} & \textbf{AUC-ROC} & \textbf{VUS-PR} & \textbf{CCE} & \textbf{F1} & \textbf{Aff-F1} & \textbf{UAff-F1} & \textbf{AUC-ROC} & \textbf{VUS-PR} & \textbf{CCE} & \textbf{F1} & \textbf{Aff-F1} & \textbf{UAff-F1} & \textbf{AUC-ROC} & \textbf{VUS-PR} \\
    \midrule
    \rowcolor[rgb]{ .949,  .949,  .949} Random & -0.27  & 8.65  & \uline{26.68 } & -0.69  & 49.79  & 83.90  & 0.72  & 1.53  & 63.75  & -3.53  & 50.32  & 3.57  & -0.18  & 6.13  & 59.31  & -1.67  & 49.99  & 28.34  \\
    \rowcolor[rgb]{ .949,  .949,  .949} IForest & 5.85  & 18.18  & 11.56  & 5.15  & 66.30  & 85.11  & 12.35  & 8.11  & 60.59  & 19.21  & 79.10  & 10.09  & 3.72  & 9.41  & 49.17  & 0.35  & 59.92  & 30.54  \\
    \rowcolor[rgb]{ .949,  .949,  .949} LOF   & 0.14  & 10.32  & 21.67  & 5.50  & 49.14  & 83.10  & 0.07  & 2.91  & 64.47  & 1.14  & 50.30  & 4.33  & 0.32  & 8.14  & 61.48  & 15.23  & 51.39  & 29.53  \\
    \rowcolor[rgb]{ .949,  .949,  .949} PCA   & 1.55  & 24.75  & 2.21  & 2.00  & 59.62  & 93.45  & 11.38  & 18.03  & 62.58  & 47.28  & 90.68  & 17.92  & 7.68  & \uline{29.89 } & 54.12  & \textbf{38.28 } & \textbf{79.05 } & \textbf{53.03 } \\
    \rowcolor[rgb]{ .949,  .949,  .949} HBOS  & \textbf{15.92 } & 18.01  & 23.08  & 20.14  & \textbf{78.82 } & 88.77  & 16.45  & 8.16  & 65.15  & 9.51  & 82.93  & 11.87  & 9.60  & 10.99  & 54.38  & 8.34  & 72.14  & 35.74  \\
    \rowcolor[rgb]{ .949,  .949,  .949} KNN   & -3.17  & 6.67  & 20.69  & -15.08  & 32.99  & 83.35  & 3.40  & 5.06  & 65.87  & 0.35  & 55.71  & 8.86  & -0.77  & 6.04  & 59.08  & 4.23  & 38.47  & 27.96  \\
    \rowcolor[rgb]{ .949,  .949,  .949} KMeans & -7.41  & 6.43  & 11.18  & 6.27  & 30.04  & 81.24  & \textbf{28.38 } & 17.89  & 72.45  & 46.33  & \textbf{92.85 } & 24.01  & 6.47  & 12.88  & 57.67  & 34.45  & 51.86  & 33.47  \\
    \midrule
        \midrule
    \rowcolor[rgb]{ .886,  .937,  .855} OCSVM & \uline{11.82 } & 10.43  & 10.96  & 8.70  & 71.10  & 85.26  & \uline{20.57 } & 17.79  & 70.93  & 20.01  & \uline{92.31 } & 22.78  & \textbf{11.74 } & 16.43  & 46.95  & 25.63  & 75.04  & 40.66  \\
    \rowcolor[rgb]{ .886,  .937,  .855} AE    & 5.95  & 18.91  & 21.89  & \uline{20.80 } & 60.01  & 88.57  & 1.76  & 5.68  & 54.44  & 22.81  & 50.71  & 2.36  & 9.36  & 14.93  & 56.41  & \uline{35.46 } & 63.26  & 37.51  \\
    \rowcolor[rgb]{ .886,  .937,  .855} CNN   & 0.56  & 24.84  & 15.92  & 15.78  & 72.99  & 93.71  & 2.62  & 3.96  & 44.78  & 9.19  & 54.04  & 2.55  & 7.04  & 27.53  & 42.78  & 26.79  & 68.23  & 46.72  \\
    \rowcolor[rgb]{ .886,  .937,  .855} LSTM  & 0.38  & 23.98  & \textbf{27.41 } & \textbf{27.11 } & 75.24  & 92.63  & 2.62  & 8.63  & 54.09  & 12.65  & 60.35  & 5.84  & 7.12  & 28.36  & 46.42  & 29.14  & 71.38  & \uline{48.92 } \\
    \rowcolor[rgb]{ .886,  .937,  .855} TranAD & 0.08  & 15.94  & 18.57  & 5.76  & 65.01  & 91.96  & 0.32  & 6.20  & 50.82  & 13.96  & 52.11  & 6.51  & 6.60  & 24.76  & 43.21  & 24.69  & 67.78  & 47.82  \\
    \rowcolor[rgb]{ .886,  .937,  .855} USAD  & 0.54  & 20.85  & 11.95  & 11.42  & 61.81  & 92.27  & 3.21  & 9.35  & 41.21  & 13.84  & 71.66  & 6.27  & 8.68  & 26.59  & 36.49  & 23.07  & 71.46  & 47.25  \\
    \rowcolor[rgb]{ .886,  .937,  .855} Omni  & 1.86  & 24.44  & 0.26  & -0.25  & 68.55  & \uline{94.25 } & 3.23  & 9.30  & 41.19  & 5.74  & 74.37  & 6.44  & \uline{9.93 } & \textbf{30.58 } & 28.45  & 17.29  & 75.00  & 48.67  \\
    \rowcolor[rgb]{ .886,  .937,  .855} A.T.  & 0.02  & 3.45  & 6.64  & -5.31  & 50.27  & 84.22  & 1.91  & 3.29  & 71.44  & 30.10  & 65.94  & 5.02  & 7.23  & 22.26  & 41.24  & 18.94  & 62.34  & 40.02  \\
    \rowcolor[rgb]{ .886,  .937,  .855} TimesNet & 0.40  & 18.79  & 12.21  & 3.41  & 58.88  & 92.56  & 0.25  & 10.11  & 63.76  & -4.59  & 71.46  & 19.50  & 0.28  & 13.95  & 59.54  & 16.73  & 57.55  & 38.15  \\
    \rowcolor[rgb]{ .886,  .937,  .855} M2N2  & 0.42  & \textbf{26.50 } & 0.03  & 0.03  & \uline{77.54 } & \textbf{96.62 } & 0.65  & \textbf{22.13 } & \textbf{84.87 } & \textbf{63.64 } & 91.91  & \textbf{37.77 } & 0.54  & 21.73  & \uline{62.91 } & 35.18  & \uline{75.67 } & 47.62  \\
    \rowcolor[rgb]{ .886,  .937,  .855} LFTSAD & 0.17  & 10.73  & 15.32  & 3.05  & 51.44  & 84.95  & 0.47  & 4.91  & 69.24  & 8.06  & 45.73  & 6.68  & 0.28  & 10.85  & 53.40  & 0.79  & 51.25  & 31.79  \\
    \rowcolor[rgb]{ .886,  .937,  .855} CATCH & 0.22  & \uline{25.60 } & 3.05  & 3.03  & 61.55  & 94.17  & 0.88  & \uline{18.98 } & \uline{81.54 } & \uline{54.51 } & 91.28  & \uline{27.36 } & 0.40  & 16.88  & \textbf{63.55 } & 35.19  & 62.61  & 41.31  \\
    \bottomrule
    \end{tabular}
    }
  \label{tab:comparison_utad}%
\end{table*}%
\begin{figure*}[htb!]
    \centering
    \resizebox{0.9\linewidth}{!}{
    \subfloat[]{\includegraphics[width=1\linewidth]{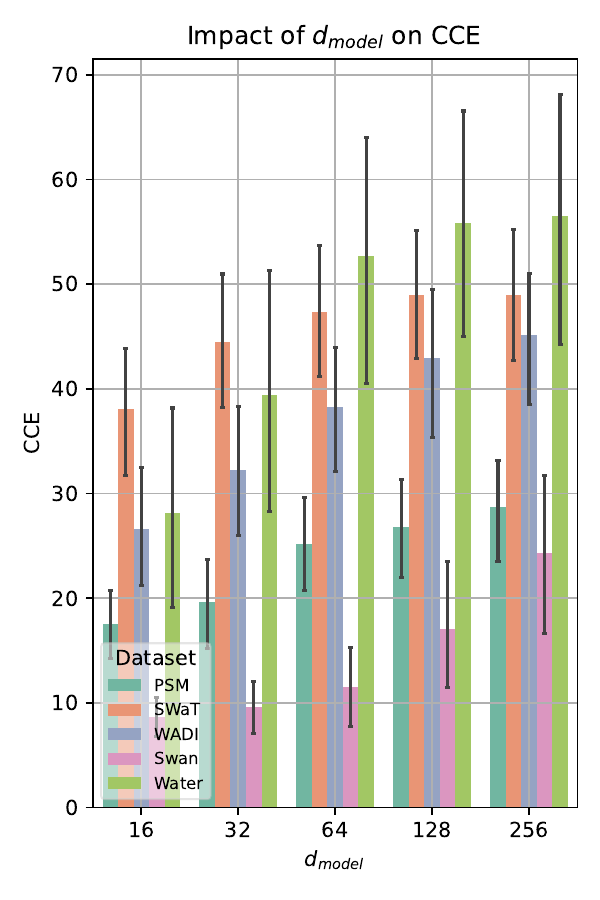}}
    \subfloat[]{\includegraphics[width=1\linewidth]{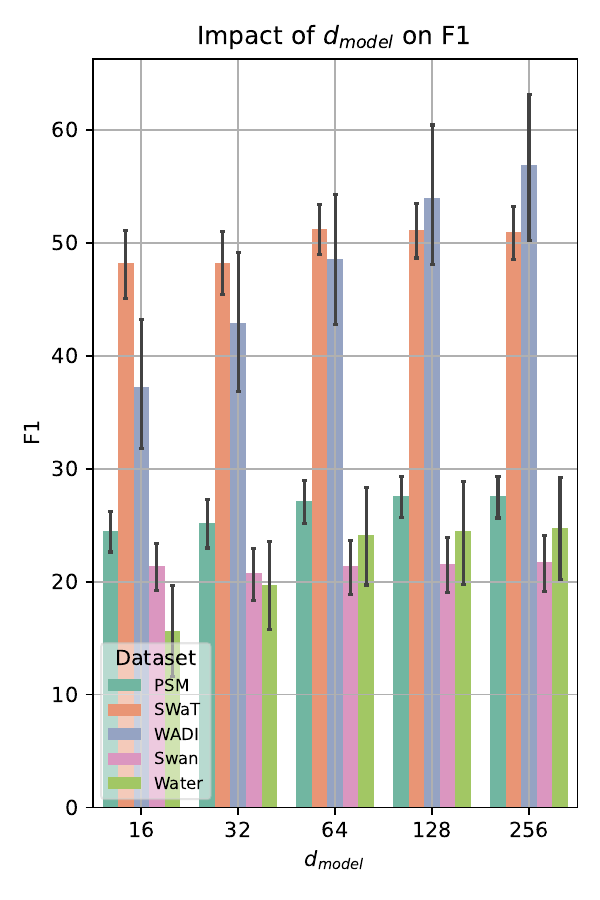}}
    \subfloat[]{\includegraphics[width=1\linewidth]{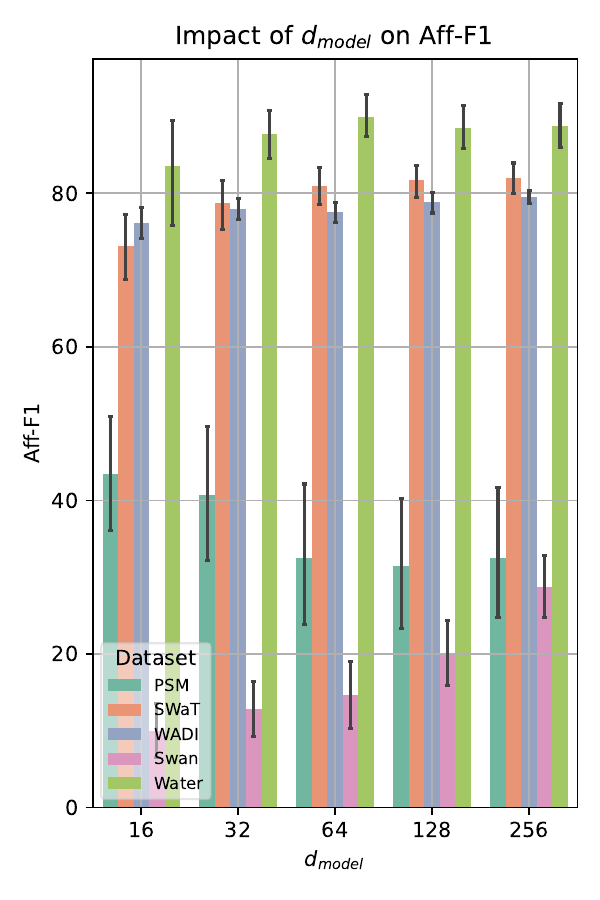}}
    \subfloat[]{\includegraphics[width=1\linewidth]{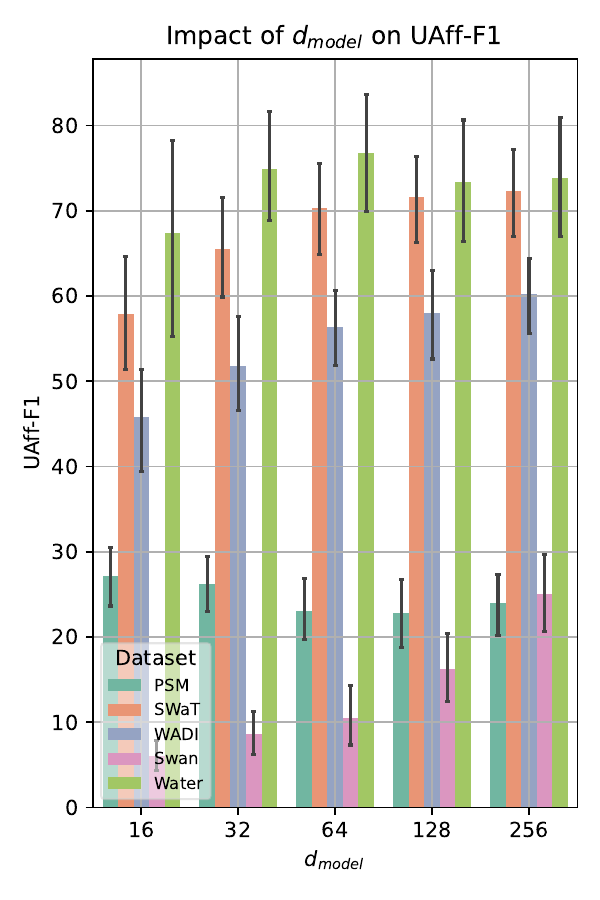}}
    \subfloat[]{\includegraphics[width=1\linewidth]{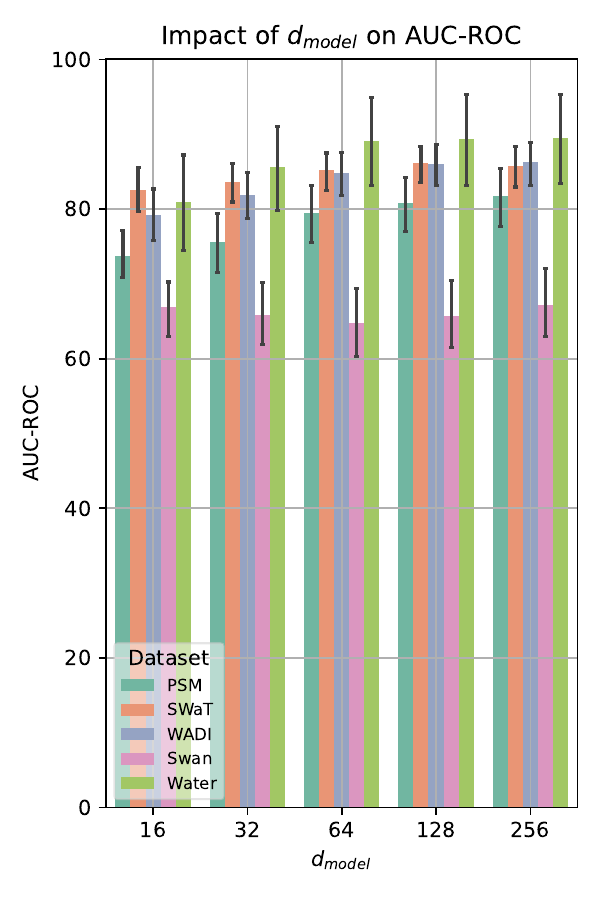}}
    \subfloat[]{\includegraphics[width=1\linewidth]{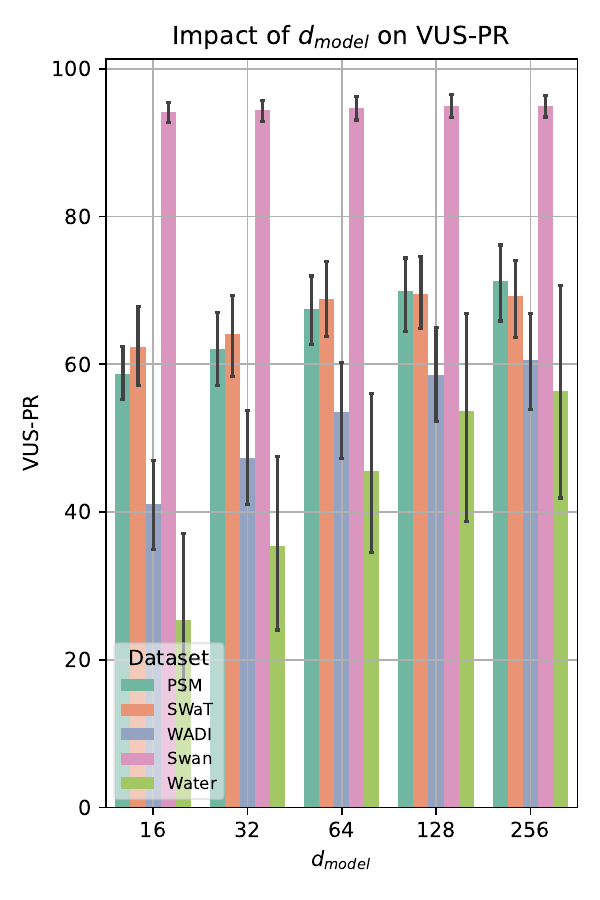}}
    }
    \caption{Sensitivity analysis of \(d_{\text{model}}\) across 5 datasets on six key performance metrics. (a) CCE; (b) F1 score; (c) Aff-F1 score (Aff-F1); (d) UAff-F1 score; (e) AUC-ROC; (f) VUS-PR. }
    \label{fig:sen_dmodel1}
\end{figure*}
\begin{figure*}[htb!]
    \centering
    \resizebox{0.9\linewidth}{!}{
    \subfloat[]{\includegraphics[width=1\linewidth]{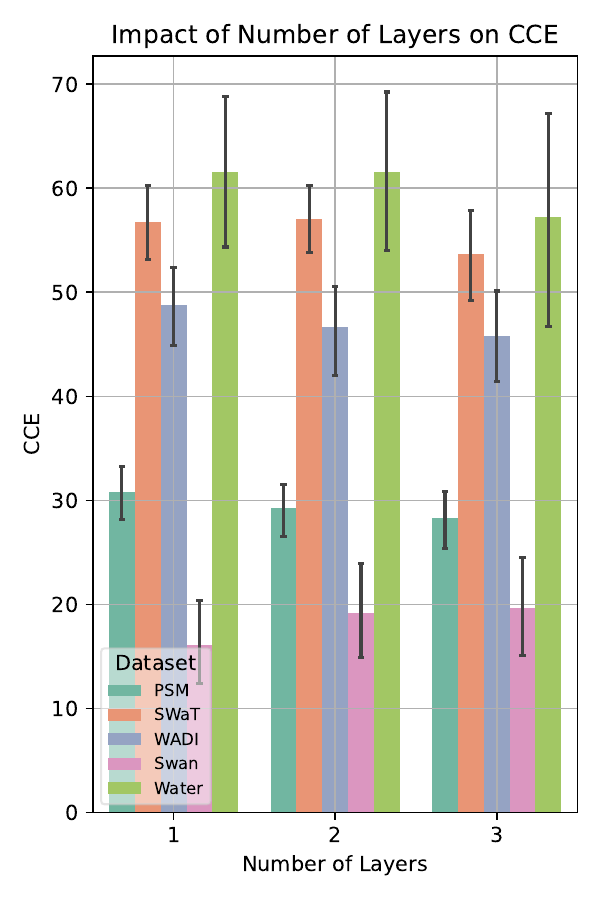}}
    \subfloat[]{\includegraphics[width=1\linewidth]{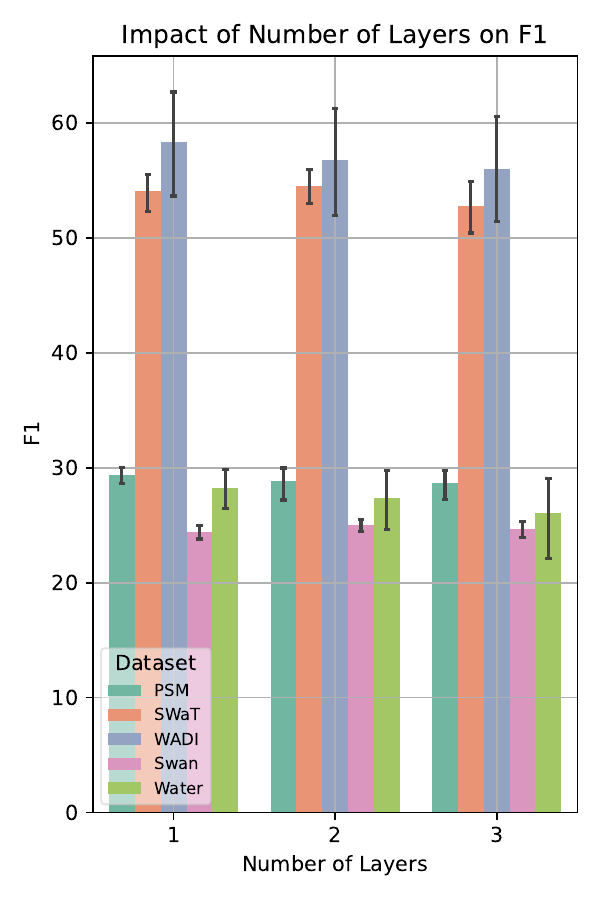}}
    \subfloat[]{\includegraphics[width=1\linewidth]{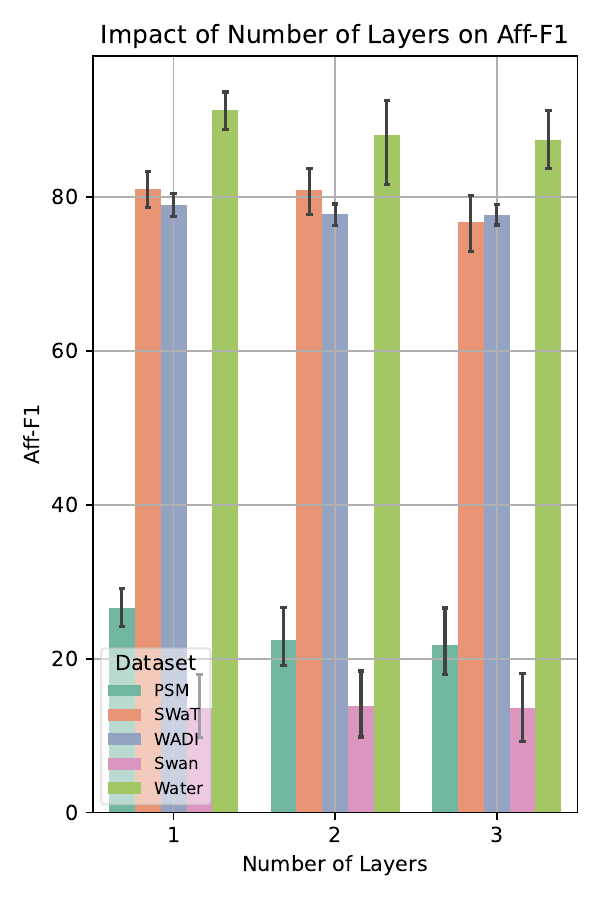}}
    \subfloat[]{\includegraphics[width=1\linewidth]{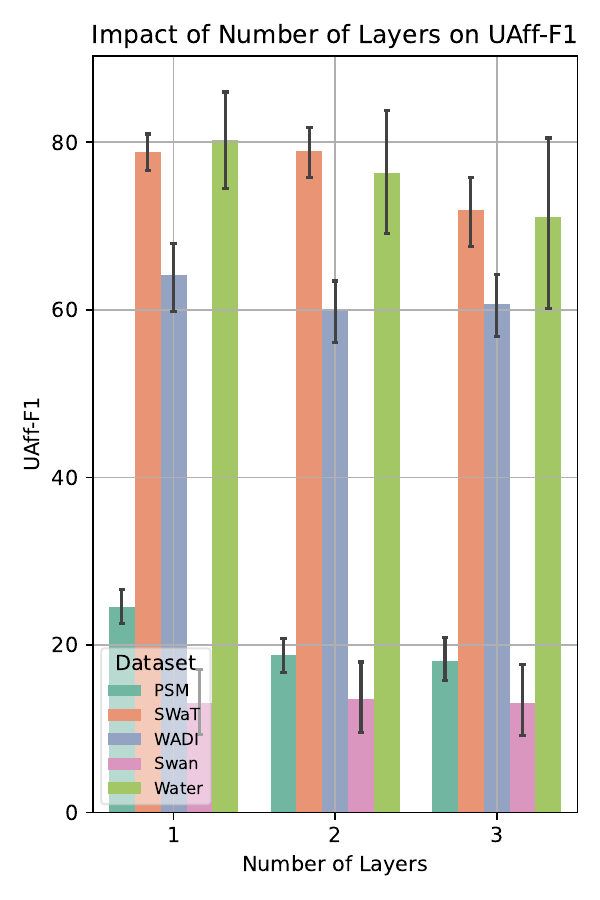}}
    \subfloat[]{\includegraphics[width=1\linewidth]{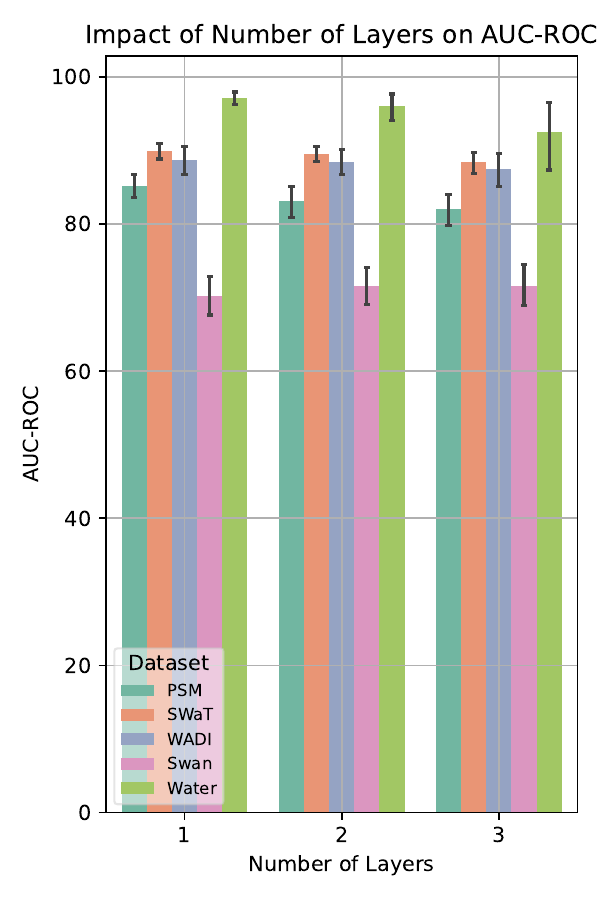}}
    \subfloat[]{\includegraphics[width=1\linewidth]{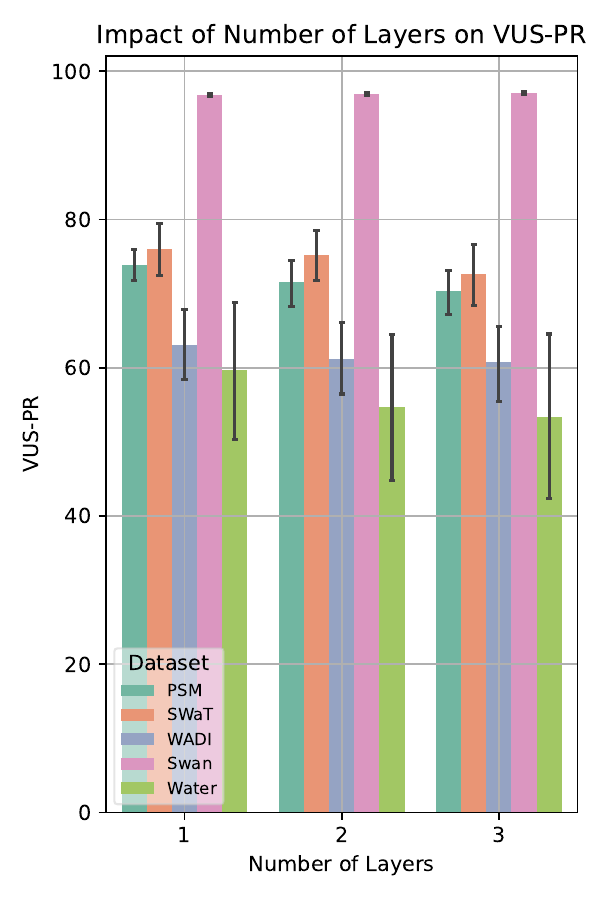}}
    }
    \caption{Sensitivity analysis of number of TEM layers  across 5 datasets on six key performance metrics. (a) CCE; (b) F1 score; (c) Aff-F1 score (Aff-F1); (d) UAff-F1 score; (e) AUC-ROC; (f) VUS-PR. }
    \label{fig:sen_tem1}
\end{figure*}
\begin{figure*}[htb!]
    \centering
    \resizebox{0.9\linewidth}{!}{
    \subfloat[]{\includegraphics[width=1\linewidth]{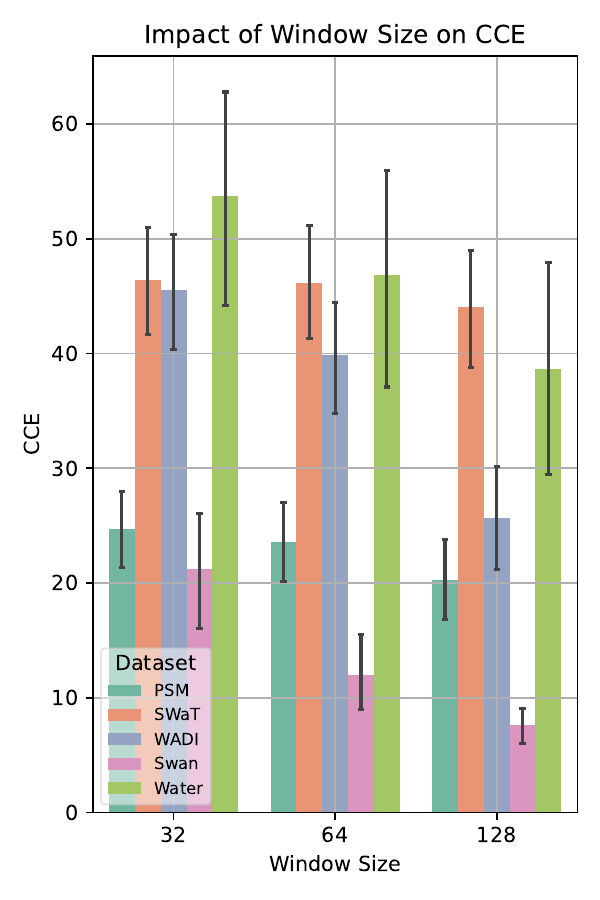}}
    \subfloat[]{\includegraphics[width=1\linewidth]{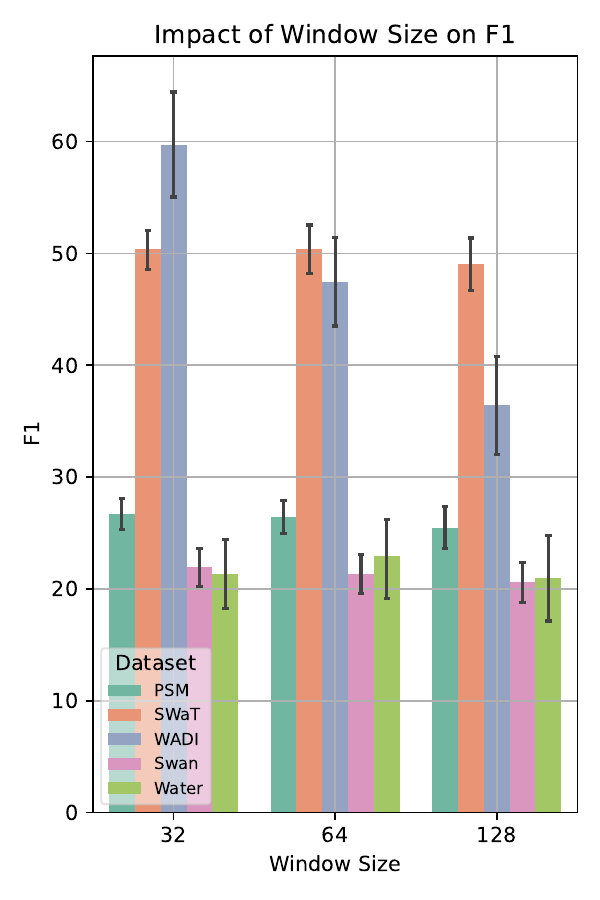}}
    \subfloat[]{\includegraphics[width=1\linewidth]{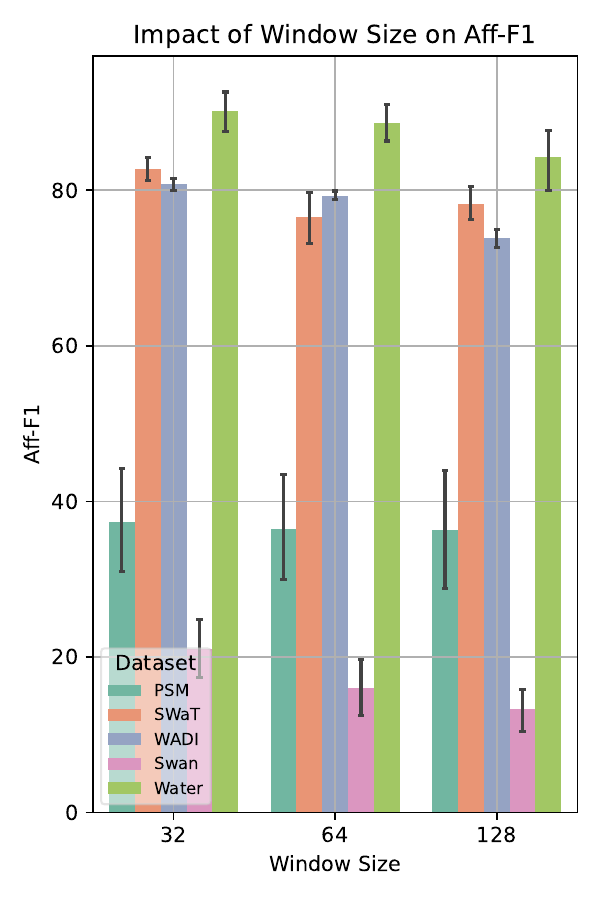}}
    \subfloat[]{\includegraphics[width=1\linewidth]{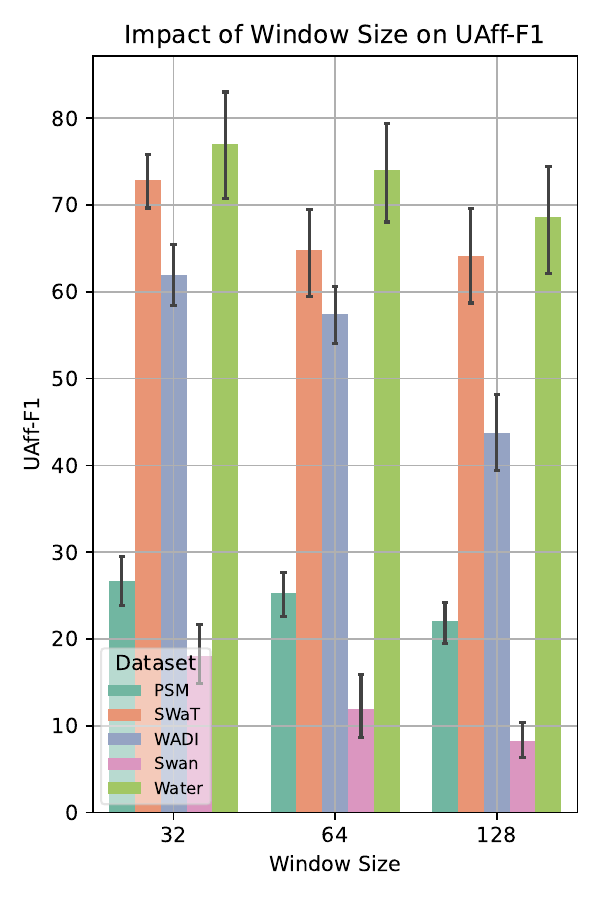}}
    \subfloat[]{\includegraphics[width=1\linewidth]{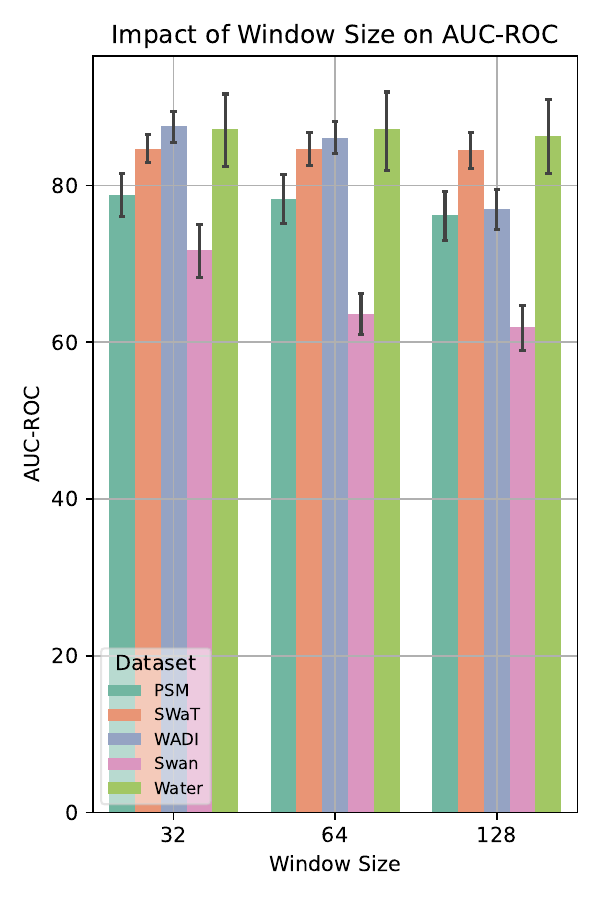}}
    \subfloat[]{\includegraphics[width=1\linewidth]{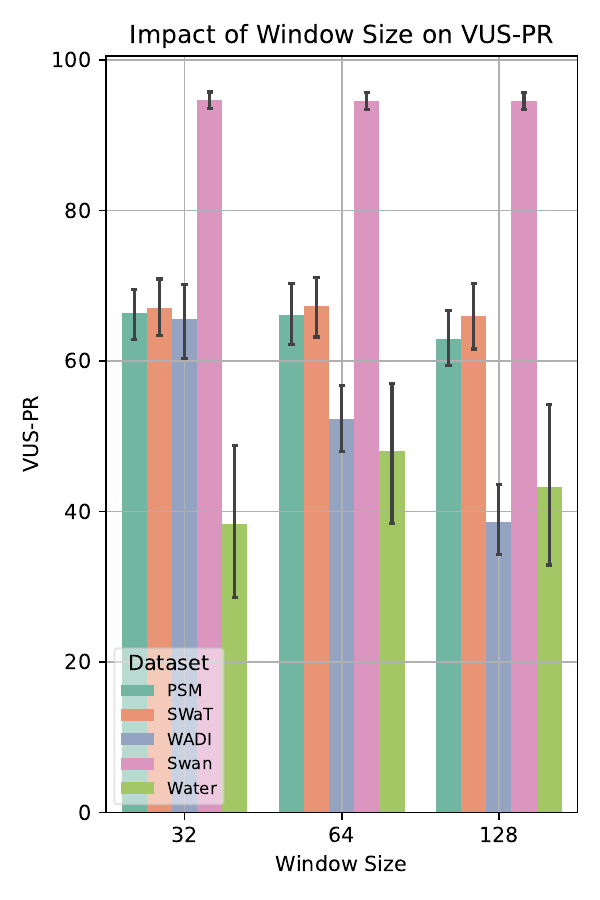}}
    }
    \caption{Sensitivity analysis of window size across 5 datasets on six key performance metrics. (a) CCE; (b) F1 score; (c) Aff-F1 score (Aff-F1); (d) UAff-F1 score; (e) AUC-ROC; (f) VUS-PR. }
    \label{fig:win_size_all1}
\end{figure*}
\begin{figure*}[htb!]
    \centering
    \resizebox{0.9\linewidth}{!}{
    \subfloat[]{\includegraphics[width=1\linewidth]{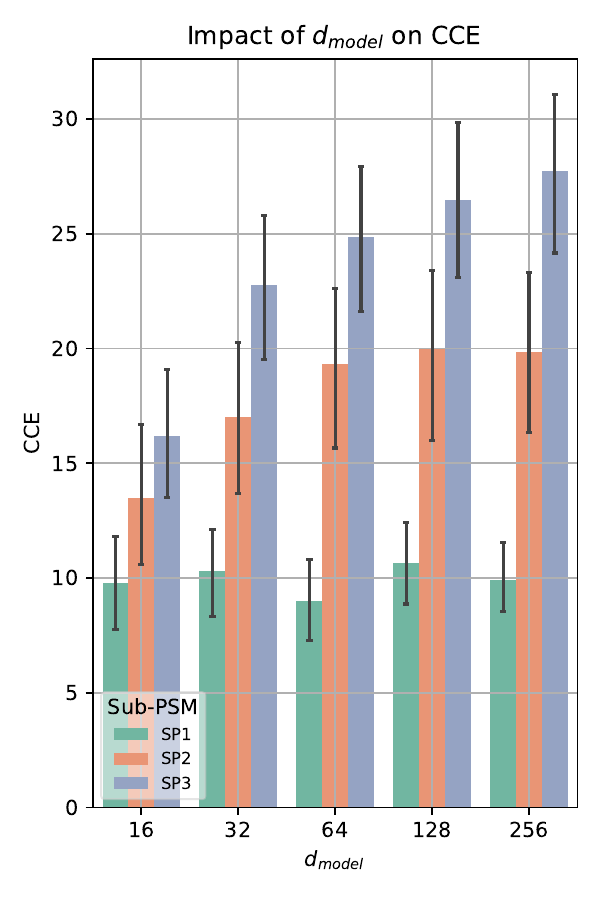}}
    \subfloat[]{\includegraphics[width=1\linewidth]{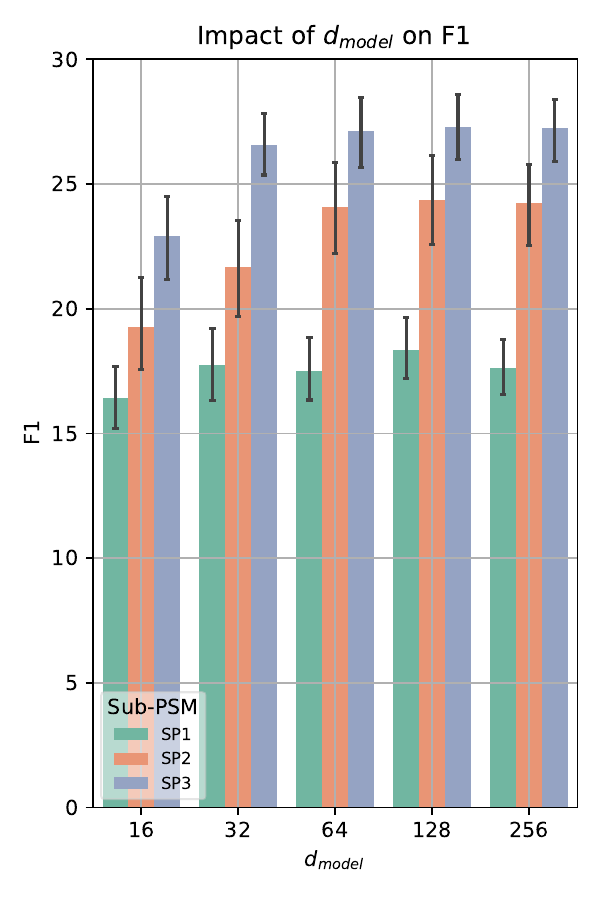}}
    \subfloat[]{\includegraphics[width=1\linewidth]{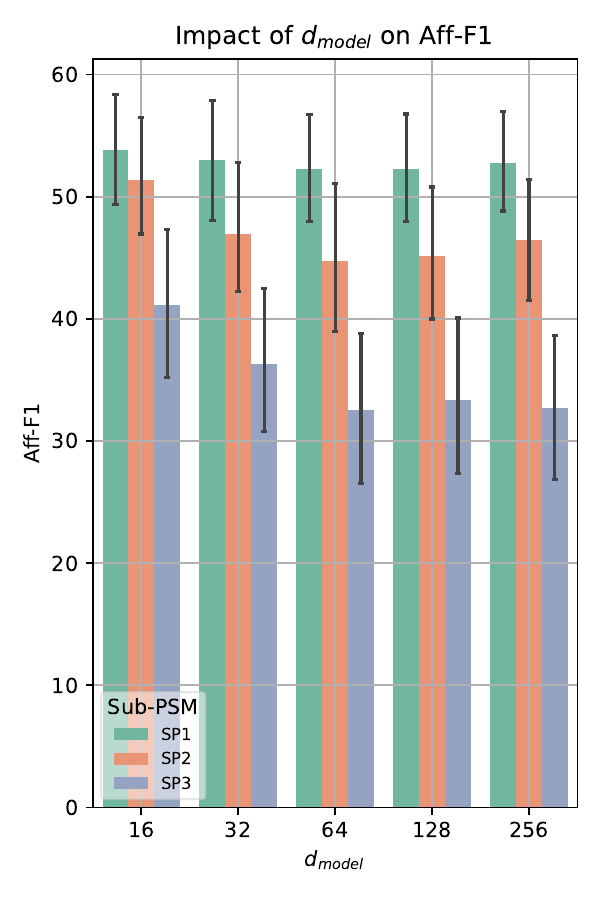}}
    \subfloat[]{\includegraphics[width=1\linewidth]{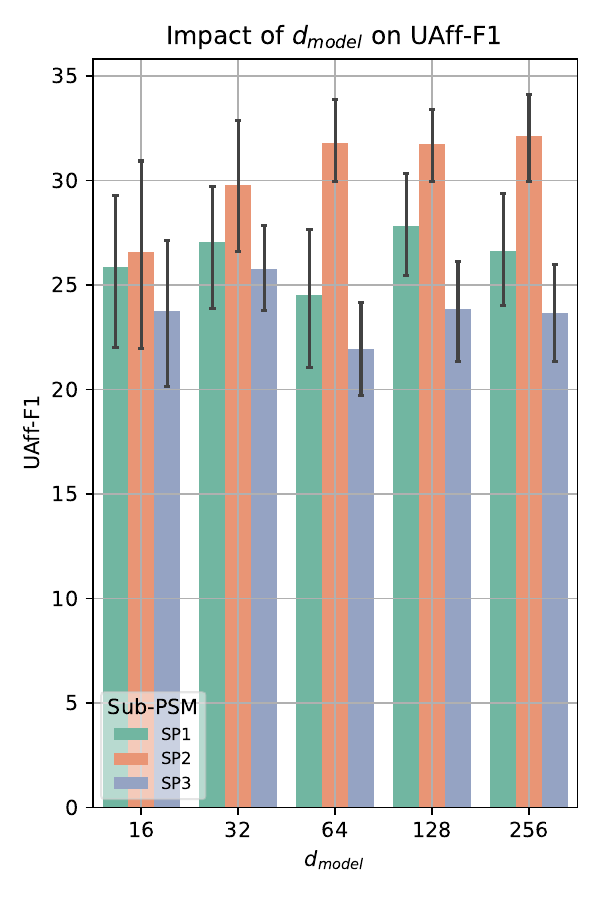}}
    \subfloat[]{\includegraphics[width=1\linewidth]{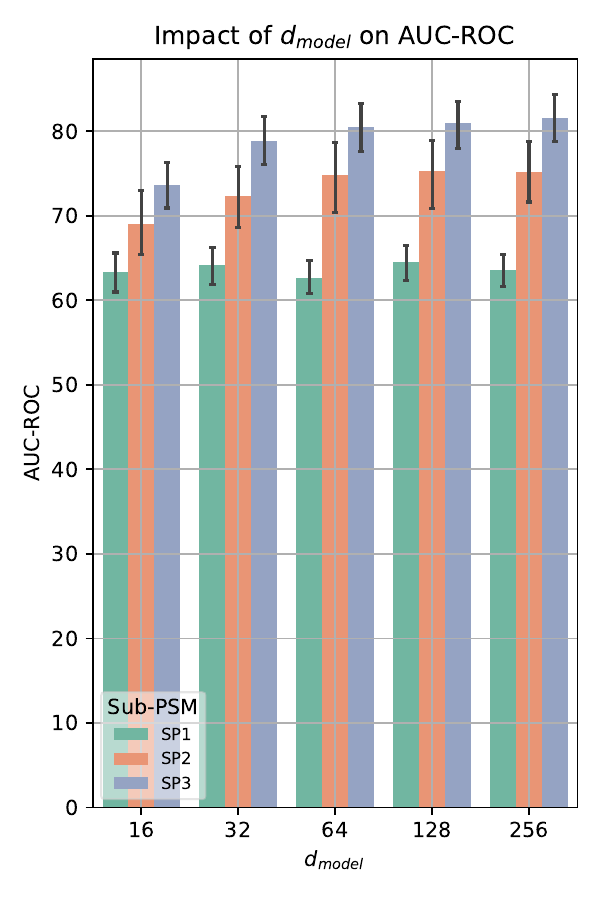}}
    \subfloat[]{\includegraphics[width=1\linewidth]{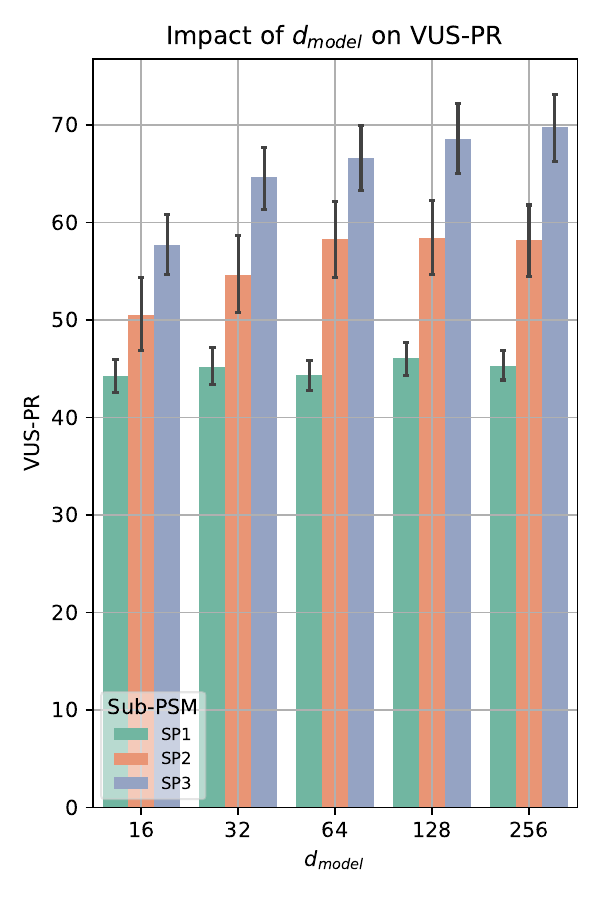}}
    }
    \caption{Sensitivity analysis of model dimension \(d_{\text{model}}\) across 4 subsets of the PSM dataset on six key performance metrics. (a) CCE; (b) F1 score; (c) Aff-F1 score (Aff-F1); (d) UAff-F1 score; (e) AUC-ROC; (f) VUS-PR. }
    \label{fig:sen_dmodel2}
\end{figure*}
\begin{figure*}[htb!]
    \centering
    \resizebox{0.9\linewidth}{!}{
    \subfloat[]{\includegraphics[width=1\linewidth]{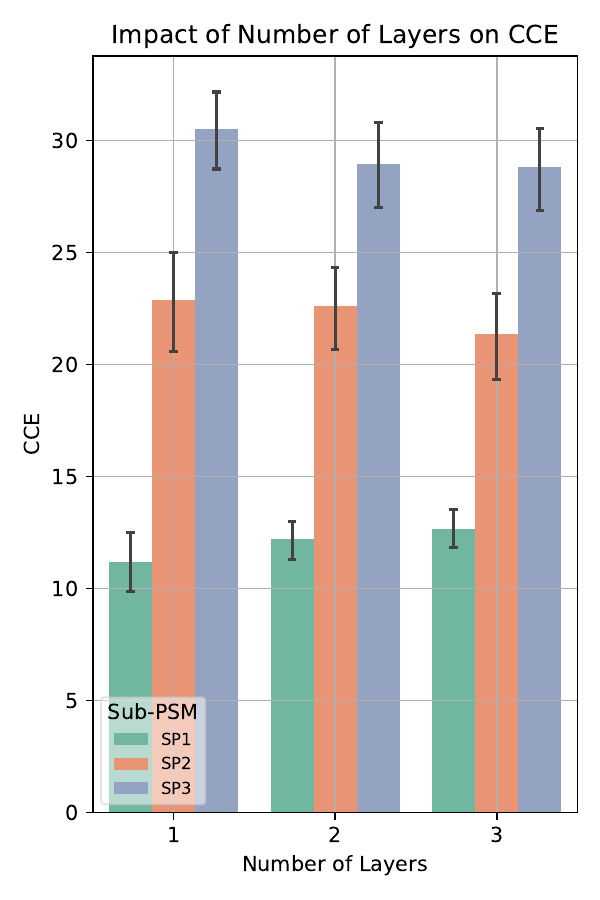}}
    \subfloat[]{\includegraphics[width=1\linewidth]{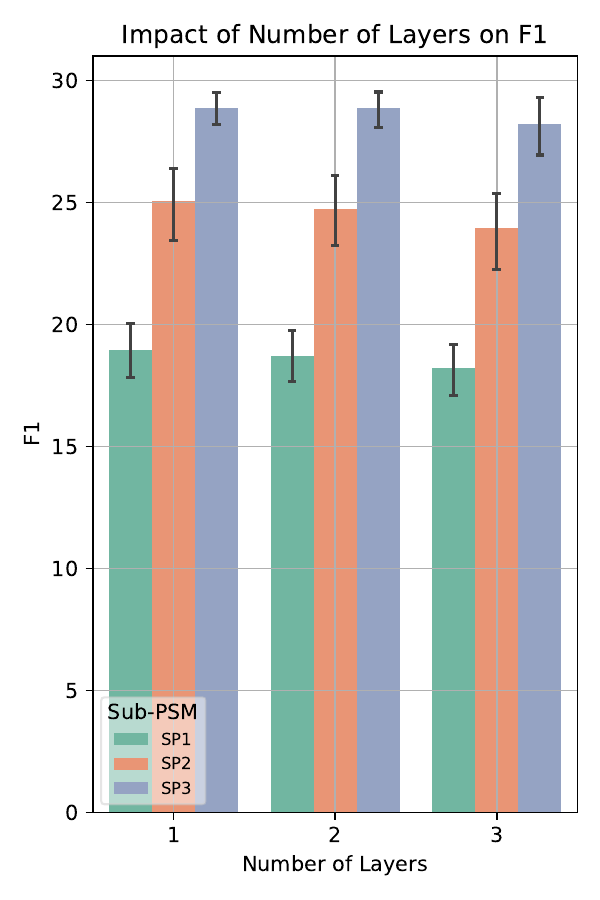}}
    \subfloat[]{\includegraphics[width=1\linewidth]{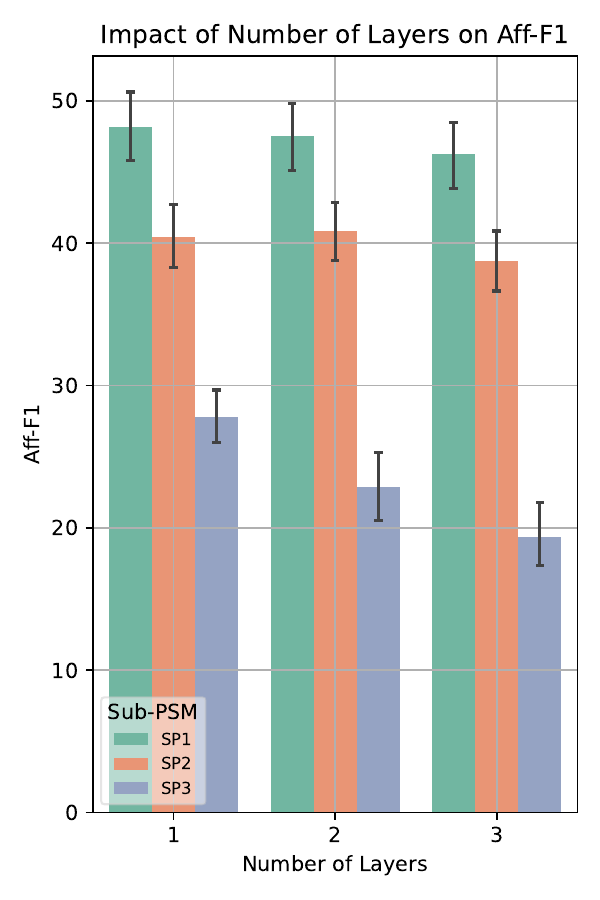}}
    \subfloat[]{\includegraphics[width=1\linewidth]{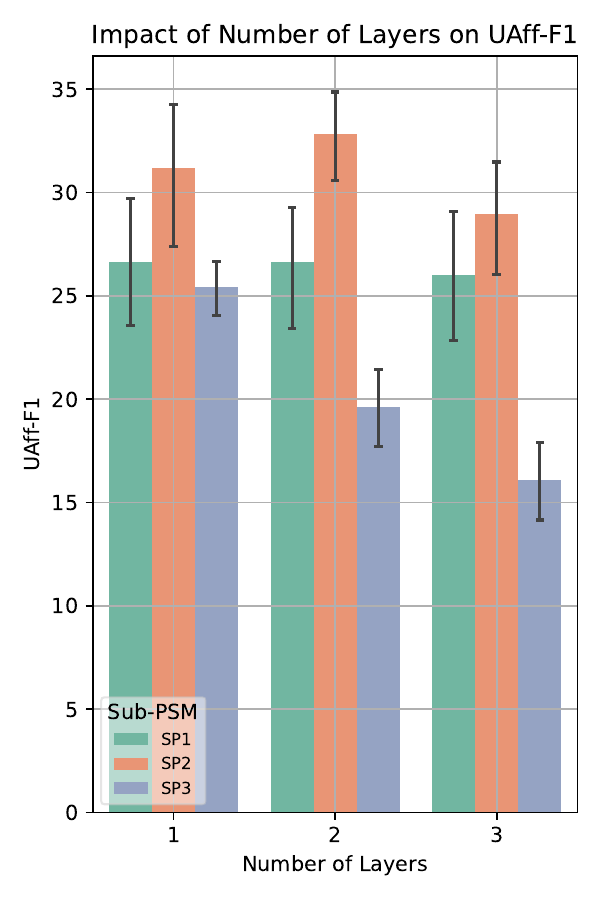}}
    \subfloat[]{\includegraphics[width=1\linewidth]{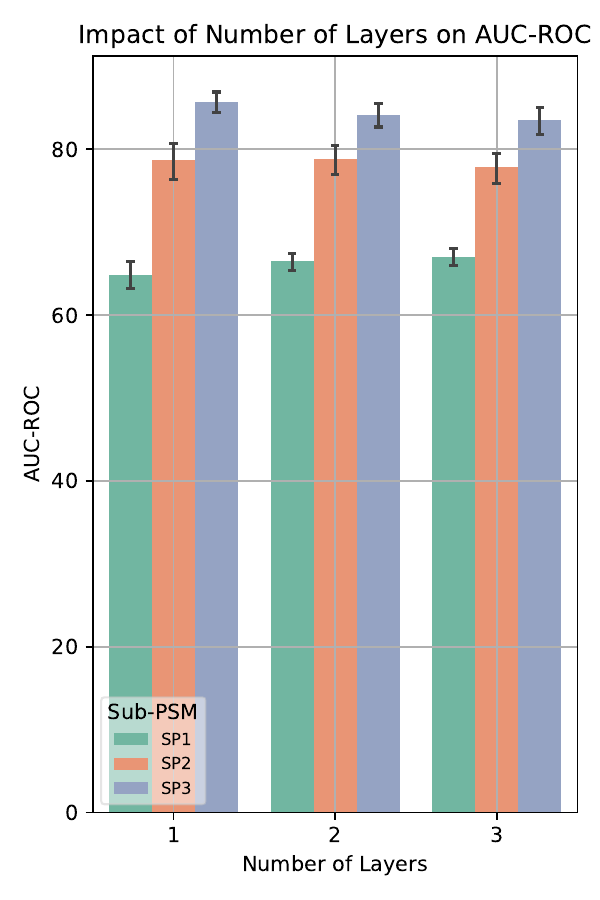}}
    \subfloat[]{\includegraphics[width=1\linewidth]{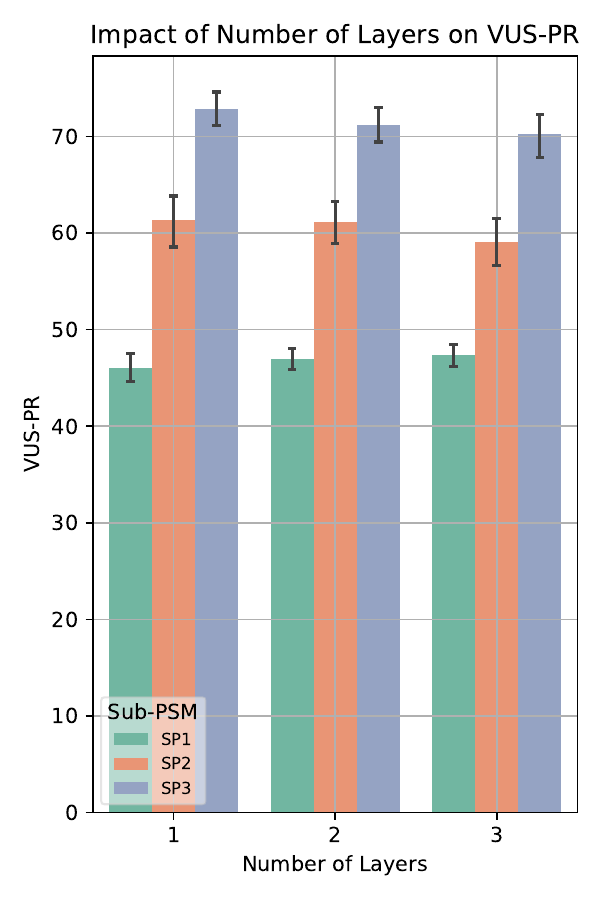}}
    }
    \caption{Sensitivity analysis of number of TEM layers across 4 subsets of the PSM dataset on six key performance metrics. (a) CCE; (b) F1 score; (c) Aff-F1 score (Aff-F1); (d) UAff-F1 score; (e) AUC-ROC; (f) VUS-PR. }
    \label{fig:tem_all2}
\end{figure*}
\begin{figure*}[htb!]
    \centering
    \resizebox{0.9\linewidth}{!}{
    \subfloat[]{\includegraphics[width=1\linewidth]{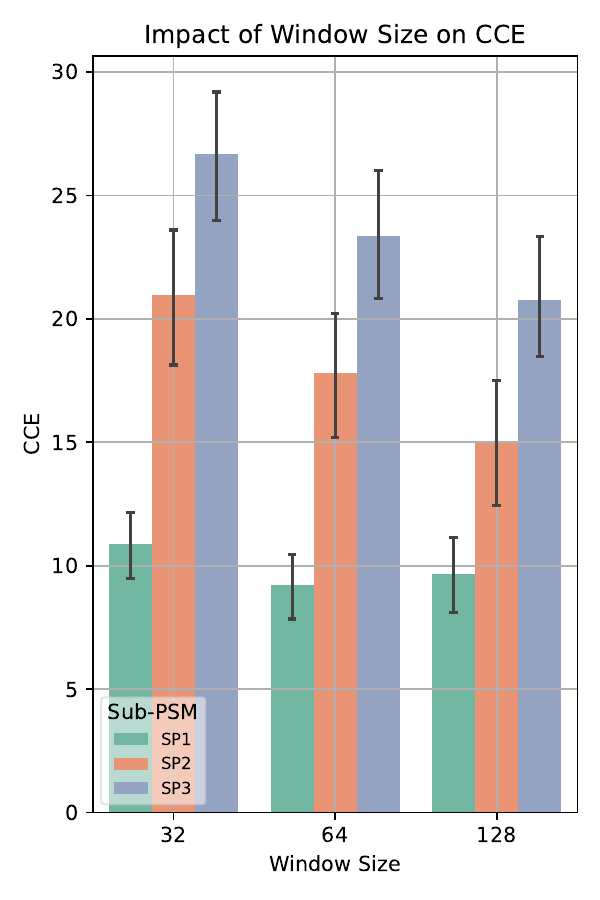}}
    \subfloat[]{\includegraphics[width=1\linewidth]{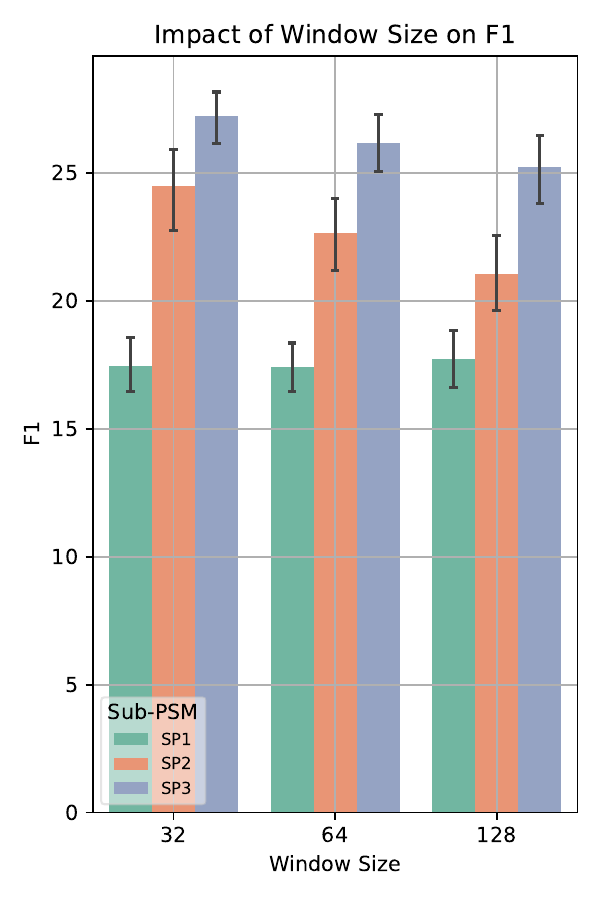}}
    \subfloat[]{\includegraphics[width=1\linewidth]{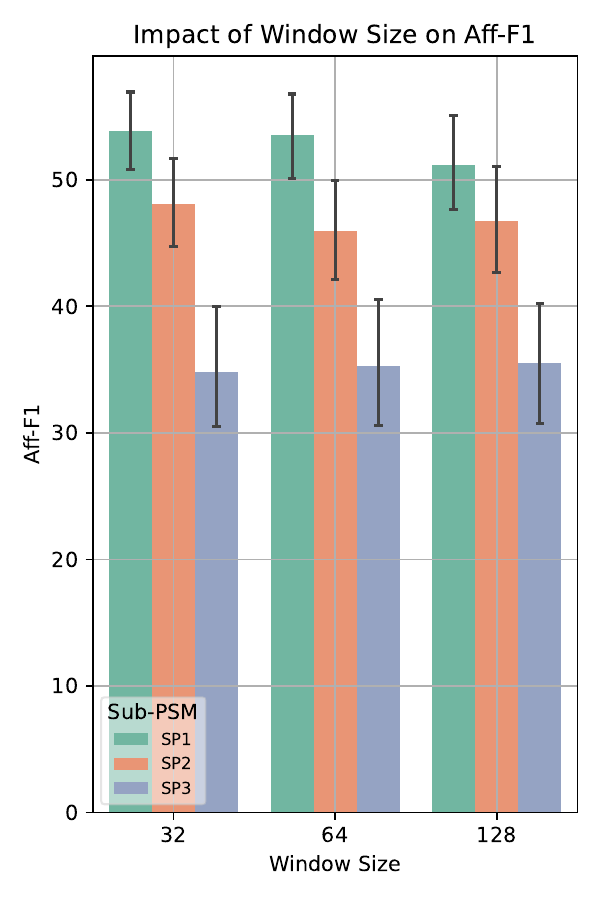}}
    \subfloat[]{\includegraphics[width=1\linewidth]{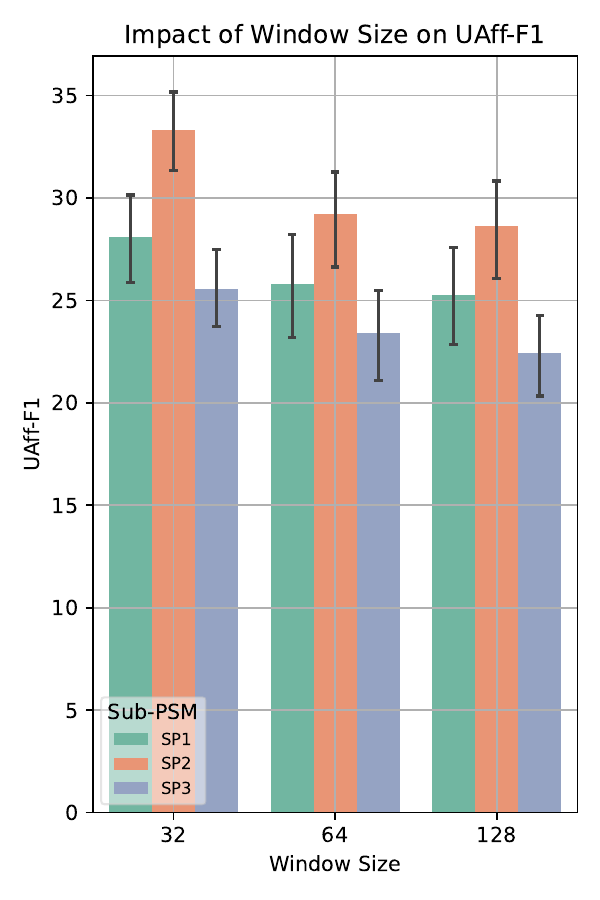}}
    \subfloat[]{\includegraphics[width=1\linewidth]{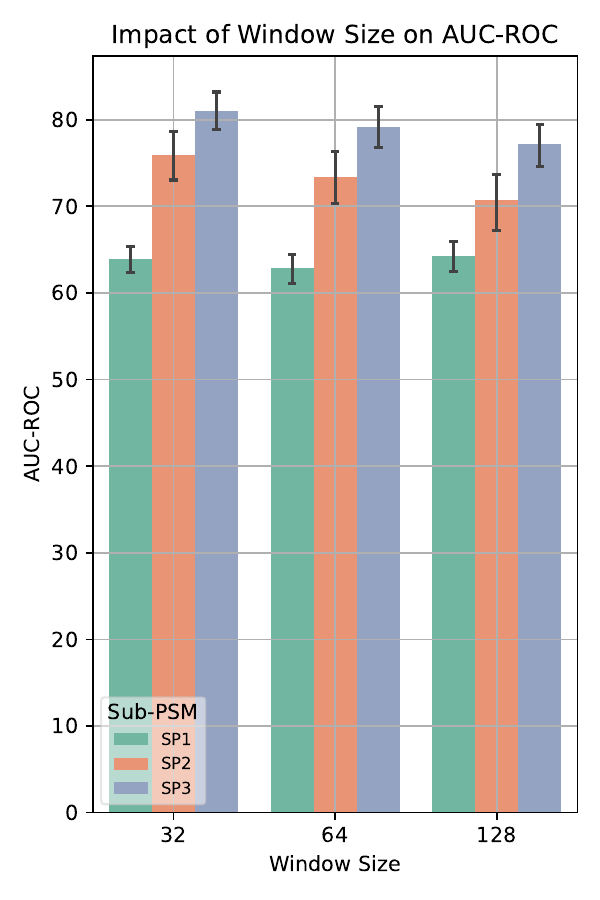}}
    \subfloat[]{\includegraphics[width=1\linewidth]{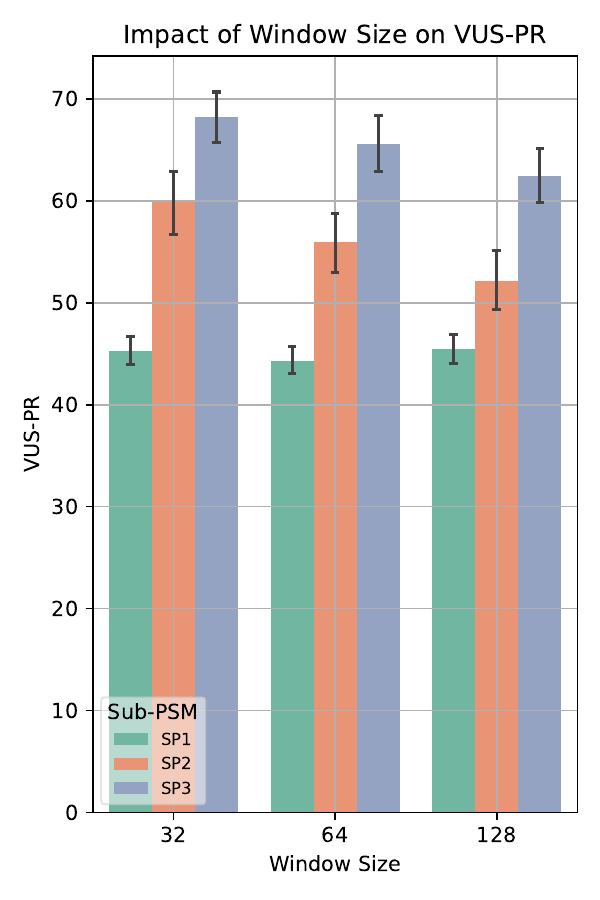}}
    }
    \caption{Sensitivity analysis of window size across 4 subsets of the PSM dataset on six key performance metrics. (a) CCE; (b) F1 score; (c) Aff-F1 score (Aff-F1); (d) UAff-F1 score; (e) AUC-ROC; (f) VUS-PR. }
    \label{fig:win_size_all2}
\end{figure*}

\section{Temporal Split Validation Results}\label{app:split_validation}
% 由于有监督方法使用了原本测试集的前半部分数据作为训练集，这导致难以公平地分析STAD方法是否真的比UTAD方法表现更好。为了缓解这一缺陷，我们在原本测试集划分后的后半部分作为真正的测试集，在这一数据集上同时测试UTAD与STAD方法，结果如表\ref{tab:left_test}所示。
% 在公平的比较下，UTAD-I中表现最好的方法是PCA，平均分数为44.34，UTAD-II中表现最好的方法是LSTM，平均分数为47.09；最新的M2N2，LFTSAD和CATCH的平均分数分别为37.91，27.96和35.71。STAD中表现最好的两个方法是RF和\stand~，平均分数分别为45.79和54.68.
% 我们发现，简单的两个STAD方法好于大部分UTAD方法，并\stand的表现远远好于其他两类方法。同时，最新的UTAD-II方法（M2N2，LFTSAD和CATCH）反而没有早期的简单方法（PCA和LSTAM）有竞争力。此外，所有UTAD方法的预测一致性（CCE）表现都较差，远远不如STAD方法，这表现它们的实际可用性不足。
Since the supervised methods utilized the initial segment of the original test set as their training data, it is challenging to fairly analyze whether STAD methods genuinely outperform UTAD methods. To mitigate this drawback, we designate the latter segment of the original test set (after partitioning) as the true evaluation set. Both UTAD and STAD methods are tested on this specific set, and the results are presented in Table \ref{tab:left_test}.

Under this fair comparison setting, the best-performing UTAD-I method is PCA, with an average score of $44.34$. For UTAD-II, the best method is LSTM, achieving an average score of $47.09$. In contrast, recent state-of-the-art UTAD-II methods, M2N2, LFTSAD, and CATCH, yield average scores of $37.91$, $27.96$, and $35.71$, respectively. The two best-performing STAD methods are RF and \stand, with average scores of $45.79$ and $54.68$.

We observe that two simple STAD methods outperform the majority of UTAD methods, and the performance of \stand~is significantly superior to both other method categories. Furthermore, we note that recent UTAD-II methods (M2N2, LFTSAD, and CATCH) are surprisingly less competitive than older, simpler approaches (PCA and LSTM). In addition, the prediction consistency (CCE) performance of all UTAD methods is poor, falling far behind that of the STAD approaches. This suggests their limited practical applicability.
\begin{table*}[htbp]
  \centering
  % \caption{Add caption}
  \caption{Three method categories' performance comparison on the latter half of the divided dataset (across five datasets and six metrics). \textbf{Bold} indicates the best performance, and \uline{underlining} indicates the second-best performance. Methods highlighted in gray are UTAD-I, methods highlighted in green are UTAD-II, and methods highlighted in orange represent STAD methods.}
  \resizebox{\linewidth}{!}{
    \begin{tabular}{c|cccccc|cccccc|cccccc}
    \toprule
    \textbf{Dataset} & \multicolumn{6}{c|}{\textbf{PSM}}             & \multicolumn{6}{c|}{\textbf{SWaT}}            & \multicolumn{6}{c}{\textbf{WADI}} \\
    \midrule
    \textbf{Metric} & \textbf{CCE} & \textbf{F1} & \textbf{Aff-F1} & \textbf{UAff-F1} & \textbf{AUC} & \textbf{V-PR} & \textbf{CCE} & \textbf{F1} & \textbf{Aff-F1} & \textbf{UAff-F1} & \textbf{AUC} & \textbf{V-PR} & \textbf{CCE} & \textbf{F1} & \textbf{Aff-F1} & \textbf{UAff-F1} & \textbf{AUC} & \textbf{V-PR} \\
    \midrule
    \rowcolor[rgb]{ .949,  .949,  .949} Random & -0.52  & 8.49  & 71.43  & 11.66  & 50.20  & 35.30  & -0.46  & 7.87  & 69.35  & -4.59  & 50.06  & 19.55  & 0.99  & 3.18  & 66.37  & 20.87  & 51.02  & 6.17  \\
    \rowcolor[rgb]{ .949,  .949,  .949} IForest & 0.40  & 14.23  & 49.22  & -1.25  & 51.34  & 36.30  & 0.40  & 6.72  & 67.58  & -3.93  & 32.17  & 15.36  & 11.57  & 10.59  & 72.41  & 26.20  & 85.22  & 19.86  \\
    \rowcolor[rgb]{ .949,  .949,  .949} LOF   & 0.84  & 11.90  & 77.47  & 29.69  & 52.37  & 39.09  & 0.07  & 7.34  & 72.47  & 11.62  & 49.90  & 19.73  & 1.16  & 7.94  & 73.75  & 27.64  & 54.82  & 8.02  \\
    \rowcolor[rgb]{ .949,  .949,  .949} PCA   & 10.22  & 17.77  & 56.73  & 51.31  & 78.32  & 59.91  & 5.64  & 34.75  & 61.50  & -2.99  & 92.11  & 77.11  & 16.32  & 32.83  & 83.96  & 58.69  & 84.93  & 29.05  \\
    \rowcolor[rgb]{ .949,  .949,  .949} HBOS  & -0.50  & 10.66  & 54.69  & 8.80  & 48.40  & 34.71  & 14.58  & 5.07  & 71.07  & 26.69  & 85.23  & 51.92  & 16.01  & 18.53  & 75.88  & 35.34  & 85.02  & 26.56  \\
    \rowcolor[rgb]{ .949,  .949,  .949} KNN   & -1.87  & 6.01  & 70.79  & 38.02  & 30.14  & 26.60  & -2.94  & 1.93  & 67.76  & -2.78  & 9.41  & 11.14  & -0.12  & 3.04  & 68.35  & -28.87  & 57.96  & 8.82  \\
    \rowcolor[rgb]{ .949,  .949,  .949} KMeans & -1.10  & 6.79  & 63.80  & 53.36  & 35.30  & 28.84  & 0.53  & 14.31  & \textbf{77.65 } & 40.88  & 21.37  & 17.78  & 13.50  & 5.43  & 60.69  & 0.36  & 73.85  & 10.92  \\
    \midrule
        \midrule
    \rowcolor[rgb]{ .886,  .937,  .855} OCSVM & -0.60  & 7.66  & 52.24  & 41.95  & 41.82  & 31.52  & 10.49  & 15.86  & 40.40  & 19.28  & 86.41  & 45.01  & 20.36  & 26.60  & 70.09  & 38.04  & \uline{90.25 } & 30.55  \\
    \rowcolor[rgb]{ .886,  .937,  .855} AE    & 5.94  & 4.90  & 35.00  & 14.38  & 59.18  & 37.57  & 21.36  & 31.37  & 76.01  & 46.24  & 91.72  & 76.31  & 22.08  & 24.35  & 73.78  & 45.87  & 77.90  & 18.94  \\
    \rowcolor[rgb]{ .886,  .937,  .855} CNN   & 2.06  & \uline{24.97 } & 49.02  & 28.51  & 78.98  & \textbf{62.25 } & 37.30  & \uline{41.57 } & 11.57  & 11.57  & 91.75  & \textbf{82.35 } & 13.53  & 28.86  & \uline{86.69 } & 64.58  & 87.09  & 35.37  \\
    \rowcolor[rgb]{ .886,  .937,  .855} LSTM  & 1.87  & \textbf{25.54 } & 53.94  & 37.36  & 77.35  & \uline{61.26 } & 38.07  & \uline{41.57 } & 12.29  & 12.29  & 89.88  & \uline{81.90 } & 14.65  & 29.25  & 86.66  & 66.06  & 83.47  & 35.49  \\
    \rowcolor[rgb]{ .886,  .937,  .855} TranAD & 0.47  & 16.40  & 47.32  & 43.45  & 69.66  & 53.91  & 38.32  & \uline{41.57 } & 12.26  & 12.26  & \uline{92.69 } & 81.38  & 12.60  & 27.93  & 85.20  & 66.75  & 84.60  & 36.17  \\
    \rowcolor[rgb]{ .886,  .937,  .855} USAD  & 4.28  & 16.72  & 44.31  & 40.91  & 72.39  & 55.40  & 38.30  & \uline{41.57 } & 12.23  & 12.23  & 92.40  & 80.85  & 15.29  & 30.31  & 86.20  & \uline{67.15 } & 76.46  & 29.52  \\
    \rowcolor[rgb]{ .886,  .937,  .855} Omni  & 11.96  & 18.16  & 17.55  & 16.05  & 72.61  & 51.57  & 38.41  & \uline{41.57 } & 11.16  & 11.16  & \textbf{92.78 } & 77.46  & 14.66  & 30.18  & 79.33  & 46.35  & 78.19  & 42.14  \\
    \rowcolor[rgb]{ .886,  .937,  .855} A.T.  & 0.51  & 10.26  & 63.57  & -3.85  & 50.65  & 36.48  & 0.00  & 1.20  & 65.24  & -14.25  & 49.26  & 19.53  & -0.34  & 1.06  & 35.84  & -53.36  & 36.60  & 5.76  \\
    \rowcolor[rgb]{ .886,  .937,  .855} TimesNet & -0.01  & 12.76  & 74.16  & 27.57  & 55.98  & 45.34  & 0.05  & 4.39  & 71.47  & 7.50  & 19.79  & 13.50  & 2.18  & 15.49  & 72.32  & 24.23  & 70.38  & 21.66  \\
    \rowcolor[rgb]{ .886,  .937,  .855} M2N2  & -0.01  & 14.83  & \uline{80.84 } & 46.18  & 65.93  & 51.71  & -0.51  & 15.32  & 27.56  & 25.80  & 80.08  & 40.06  & 10.63  & 27.13  & 81.07  & 38.19  & 83.14  & 35.44  \\
    \rowcolor[rgb]{ .886,  .937,  .855} LFTSAD & 1.02  & 18.75  & 63.38  & 28.61  & 56.44  & 44.73  & 0.73  & 22.53  & 70.22  & 3.36  & 73.46  & 45.84  & 3.30  & 14.82  & 69.27  & 34.03  & 57.60  & 13.61  \\
    \rowcolor[rgb]{ .886,  .937,  .855} CATCH & 0.54  & 15.26  & \textbf{83.83 } & \textbf{56.61 } & 61.46  & 50.61  & 0.01  & 5.79  & 72.34  & 10.56  & 19.74  & 13.57  & 2.23  & 15.75  & 76.92  & 39.90  & 80.45  & 26.05  \\
    \midrule
        \midrule
    \rowcolor[rgb]{ .988,  .894,  .839} RF    & \uline{13.14 } & 18.81  & 50.78  & 21.89  & 73.17  & 50.54  & 31.01  & 39.04  & 60.07  & \uline{56.87 } & 90.84  & 80.28  & 23.82  & \uline{46.73 } & 73.04  & 60.38  & 85.49  & \uline{63.63 } \\
    \rowcolor[rgb]{ .988,  .894,  .839} SVM   & 12.25  & 22.13  & 65.87  & 52.31  & \textbf{80.42 } & 57.39  & 19.93  & 15.09  & 68.89  & 25.96  & 91.67  & 76.17  & 12.87  & 33.22  & 81.05  & 50.59  & 81.50  & 42.92  \\
    \rowcolor[rgb]{ .988,  .894,  .839} AdaBoost & 10.05  & 20.06  & 34.14  & 28.86  & 70.80  & 39.94  & 15.39  & 22.34  & 47.91  & 34.16  & 84.07  & 37.79  & 11.60  & 27.13  & 58.41  & 24.08  & 78.62  & 27.07  \\
    \rowcolor[rgb]{ .988,  .894,  .839} ExtraTrees & 10.78  & 20.36  & 53.19  & 36.77  & \uline{79.11 } & 57.64  & 39.10  & \textbf{52.71 } & 12.91  & 12.89  & 88.88  & 53.93  & \textbf{27.43 } & \textbf{51.47 } & \textbf{88.03 } & \textbf{70.48 } & \textbf{94.61 } & \textbf{73.56 } \\
    \rowcolor[rgb]{ .988,  .894,  .839} LightGBM & 6.79  & 16.35  & 55.07  & 16.70  & 71.52  & 51.89  & \uline{39.25 } & 28.39  & 30.33  & -12.15  & 89.38  & 64.47  & 23.50  & 44.47  & 77.52  & 50.19  & 86.81  & 50.02  \\
    \rowcolor[rgb]{ .988,  .894,  .839} STAND & \textbf{16.39 } & 23.58  & 64.18  & \uline{55.61 } & 66.81  & 55.47  & \textbf{51.97 } & 36.88  & \uline{76.94 } & \textbf{69.73 } & 90.68  & 79.62  & \uline{26.70 } & 37.33  & 78.10  & 55.51  & 73.17  & 39.71  \\
    \midrule
    \textbf{Dataset} & \multicolumn{6}{c|}{\textbf{Swan}}            & \multicolumn{6}{c|}{\textbf{Water}}           & \multicolumn{6}{c}{\textbf{Average}} \\
    \midrule
    \textbf{Metric} & \textbf{CCE} & \textbf{F1} & \textbf{Aff-F1} & \textbf{UAff-F1} & \textbf{AUC} & \textbf{V-PR} & \textbf{CCE} & \textbf{F1} & \textbf{Aff-F1} & \textbf{UAff-F1} & \textbf{AUC} & \textbf{V-PR} & \textbf{CCE} & \textbf{F1} & \textbf{Aff-F1} & \textbf{UAff-F1} & \textbf{AUC} & \textbf{V-PR} \\
    \midrule
    \rowcolor[rgb]{ .949,  .949,  .949} Random & -0.10  & 9.10  & 26.79  & 4.24  & 49.71  & 89.09  & 4.74  & 0.55  & 66.75  & 0.38  & 55.06  & 0.49  & 0.93  & 5.84  & 60.14  & 6.51  & 51.21  & 30.12  \\
    \rowcolor[rgb]{ .949,  .949,  .949} IForest & 5.77  & 17.29  & 3.23  & -3.03  & 68.63  & 92.47  & 37.09  & 8.07  & 52.82  & -47.52  & 98.97  & 17.21  & 11.05  & 11.38  & 49.05  & -5.91  & 67.27  & 36.24  \\
    \rowcolor[rgb]{ .949,  .949,  .949} LOF   & 0.05  & 10.84  & 23.54  & 14.35  & 48.62  & 90.63  & 6.58  & 2.10  & 67.15  & 0.60  & 85.45  & 1.86  & 1.74  & 8.02  & \uline{62.88 } & 16.78  & 58.23  & 31.87  \\
    \rowcolor[rgb]{ .949,  .949,  .949} PCA   & 1.52  & 18.20  & 1.35  & 1.33  & 53.33  & 96.02  & 46.62  & 7.74  & 77.31  & 41.62  & 99.01  & 37.89  & 16.06  & 22.26  & 56.17  & 29.99  & 81.54  & 60.00  \\
    \rowcolor[rgb]{ .949,  .949,  .949} HBOS  & 13.70  & 15.04  & 18.22  & 13.47  & 80.02  & 96.18  & 31.77  & 6.85  & 56.58  & -39.18  & 96.26  & 9.63  & 15.11  & 11.23  & 55.29  & 9.02  & 78.99  & 43.80  \\
    \rowcolor[rgb]{ .949,  .949,  .949} KNN   & -3.79  & 7.71  & 22.44  & -15.13  & 31.37  & 88.35  & 22.65  & 4.20  & 49.15  & -52.68  & 70.61  & 5.60  & 2.79  & 4.58  & 55.70  & -12.29  & 39.90  & 28.10  \\
    \rowcolor[rgb]{ .949,  .949,  .949} KMeans & -9.32  & 4.74  & 16.58  & 8.88  & 23.50  & 87.55  & 44.24  & 6.19  & 39.83  & -66.82  & 93.74  & 24.05  & 9.57  & 7.49  & 51.71  & 7.33  & 49.55  & 33.83  \\
    \midrule
        \midrule
    \rowcolor[rgb]{ .886,  .937,  .855} OCSVM & 11.64  & 11.31  & 12.23  & 10.84  & 68.59  & 92.06  & 37.64  & 8.40  & 75.02  & 34.46  & \uline{99.35 } & 21.63  & 15.91  & 13.97  & 50.00  & 28.91  & 77.28  & 44.15  \\
    \rowcolor[rgb]{ .886,  .937,  .855} AE    & 13.97  & 13.59  & 21.21  & 20.46  & 68.29  & 92.43  & 17.22  & 1.88  & 71.53  & 22.88  & 58.07  & 2.88  & 16.11  & 15.22  & 55.51  & 29.97  & 71.03  & 45.63  \\
    \rowcolor[rgb]{ .886,  .937,  .855} CNN   & 0.69  & 18.42  & 0.08  & 0.08  & 66.83  & 96.12  & 31.41  & 8.51  & 90.19  & 78.80  & \textbf{99.87 } & \textbf{59.99 } & 17.00  & \textbf{24.47 } & 47.51  & 36.71  & \textbf{84.90 } & \textbf{67.22 } \\
    \rowcolor[rgb]{ .886,  .937,  .855} LSTM  & 0.50  & 16.37  & 29.49  & \uline{29.11 } & 71.67  & 95.29  & 27.28  & 5.31  & 93.18  & 85.62  & 91.41  & 18.73  & 16.47  & 23.61  & 55.11  & \uline{46.09 } & 82.76  & 58.53  \\
    \rowcolor[rgb]{ .886,  .937,  .855} TranAD & 0.08  & 11.20  & 19.84  & -7.58  & 60.35  & 94.03  & 19.12  & 5.20  & 91.42  & 81.54  & 94.48  & 20.85  & 14.12  & 20.46  & 51.21  & 39.28  & 80.35  & 57.27  \\
    \rowcolor[rgb]{ .886,  .937,  .855} USAD  & 0.70  & 16.44  & 3.97  & 3.81  & 56.80  & 95.05  & 29.06  & 5.53  & 90.52  & 79.71  & 93.95  & 20.92  & 17.53  & 22.11  & 47.45  & 40.76  & 78.40  & 56.35  \\
    \rowcolor[rgb]{ .886,  .937,  .855} Omni  & 2.45  & 18.34  & 0.08  & 0.08  & 59.54  & 95.63  & 18.24  & 3.98  & 92.22  & 83.31  & 92.90  & 42.93  & 17.14  & 22.45  & 40.07  & 31.39  & 79.20  & \uline{61.95 } \\
    \rowcolor[rgb]{ .886,  .937,  .855} A.T.  & 0.01  & 5.64  & 18.16  & -12.74  & 49.19  & 89.65  & 15.94  & 2.99  & 51.39  & -43.74  & 61.45  & 2.99  & 3.22  & 4.23  & 46.84  & -25.59  & 49.43  & 30.88  \\
    \rowcolor[rgb]{ .886,  .937,  .855} TimesNet & 0.59  & \uline{18.48 } & 0.08  & 0.08  & 53.38  & 94.57  & 0.98  & 3.76  & 67.92  & 10.57  & 82.65  & 25.59  & 0.76  & 10.97  & 57.19  & 13.99  & 56.44  & 40.13  \\
    \rowcolor[rgb]{ .886,  .937,  .855} M2N2  & 0.53  & 18.45  & 0.08  & 0.08  & 85.05  & \textbf{98.41 } & 7.69  & 5.64  & 70.36  & 13.77  & 91.45  & 22.53  & 3.67  & 16.27  & 51.98  & 24.80  & 81.13  & 49.63  \\
    \rowcolor[rgb]{ .886,  .937,  .855} LFTSAD & 0.09  & 12.80  & 15.11  & -5.85  & 44.97  & 90.26  & 0.11  & 1.88  & 51.36  & -46.26  & 51.50  & 1.12  & 1.05  & 14.16  & 53.87  & 2.77  & 56.79  & 39.11  \\
    \rowcolor[rgb]{ .886,  .937,  .855} CATCH & 0.40  & \uline{18.48 } & 0.08  & 0.08  & 55.82  & 95.67  & 22.06  & 5.53  & 75.30  & 32.23  & 89.20  & \uline{44.83 } & 5.05  & 12.16  & 61.69  & 27.88  & 61.33  & 46.15  \\
    \midrule
        \midrule
    \rowcolor[rgb]{ .988,  .894,  .839} RF    & 27.51  & 16.68  & \uline{29.91 } & 28.55  & \uline{87.60 } & 95.32  & \uline{53.80 } & \uline{19.66 } & 65.81  & 60.20  & 87.16  & 26.33  & \uline{26.14 } & 17.93  & 54.32  & 40.44  & 84.07  & 51.85  \\
    \rowcolor[rgb]{ .988,  .894,  .839} SVM   & 12.31  & 16.55  & 25.65  & 24.73  & 82.46  & \uline{97.19 } & 19.17  & 7.24  & 66.59  & 42.27  & 65.06  & 12.07  & 11.31  & 12.00  & 51.72  & 33.02  & 77.30  & 47.20  \\
    \rowcolor[rgb]{ .988,  .894,  .839} AdaBoost & 33.24  & \textbf{20.19 } & 27.23  & 25.98  & 87.31  & 93.06  & 33.52  & 17.43  & \textbf{98.42 } & \textbf{96.84 } & 88.12  & 32.65  & 17.59  & 14.29  & 46.72  & 28.74  & 78.36  & 45.24  \\
    \rowcolor[rgb]{ .988,  .894,  .839} ExtraTrees & 27.90  & 17.86  & 28.26  & 26.99  & 87.35  & 95.54  & 26.57  & 13.18  & \uline{97.91 } & \uline{96.04 } & 85.31  & 11.49  & 25.52  & 18.39  & 50.63  & 35.95  & \uline{84.59 } & 52.82  \\
    \rowcolor[rgb]{ .988,  .894,  .839} LightGBM & \textbf{38.09 } & 16.29  & \textbf{36.29 } & \textbf{35.21 } & \textbf{89.54 } & 94.90  & 21.21  & \textbf{26.39 } & 33.03  & -2.69  & 80.66  & 3.80  & 24.28  & 14.79  & 49.23  & 21.57  & 80.89  & 47.88  \\
    \rowcolor[rgb]{ .988,  .894,  .839} STAND & \textbf{\uline{33.26 }} & 17.17  & 27.39  & 26.95  & 77.27  & 96.69  & \textbf{64.19 } & 6.63  & 92.21  & 83.33  & 96.53  & 20.37  & \textbf{38.50 } & \uline{24.32 } & \textbf{67.76 } & \textbf{58.22 } & 80.89  & 58.37  \\
    \bottomrule
    \end{tabular}}
  \label{tab:left_test}%
\end{table*}%

\section{Full Results of STAND Sensitivity Analysis}\label{app:sen}

% 为了探究\stand 的参数敏感性，我们在五个真实数据集和4个PSM子集上都进行了参数分析。图\ref{fig:sen_dmodel1},\ref{fig:sen_tem1}和\ref{fig:win_size_all1}分别展示了模型维度，TEM层数与时间窗口大小对\stand~的影响，在5个数据上。整体而言，模型随着模型维度的增大而提升性能（几乎所有指标），模型随着TEM层数和时间窗口的增大而性能下降（点级别与事件级别指标）。

% 图\ref{fig:sen_dmodel1},\ref{fig:sen_tem1}和\ref{fig:win_size_all1}分别展示了模型维度，TEM层数与时间窗口大小对\stand~的影响，在四个PSM自己上。整体上，模型性能的变化趋势与5个真实数据集上的趋势一致。当模型维度增大时，模型在SP2-SP4三个子集上性能都得到了提升，但是在SP1上的性能变化相对更小。相反，当TEM层数与时间窗口大小增大时，模型在SP2-SP4三个子集上的性能都略微下降，但在SP1上的性能变化没有明显趋势。
% 因此超参数对\stand的影响主要体现在，数据集增大时影响严重，呈现明显的变化趋势，当数据量较少时，模型受到随机初始化的影响更严重，导致性能变化趋势并不明显。
% 此外，特别注意到，训练集为SP1时，Aff-F1和UAff-F1分数的平均水平明显好于训练集为SP2-SP4。这是因为这两个指标需要设置异常评估的缓冲区，在缓冲区部分的模型预测同样视作预测正确。当异常占比较少时，这种容忍指标容易造成不准确的评估。
To investigate the parameter sensitivity of \stand, we conducted a comprehensive parameter analysis across all five real-world datasets and the four PSM subsets.

Figures \ref{fig:sen_dmodel1}, \ref{fig:sen_tem1}, and \ref{fig:win_size_all1} illustrate the impact of the model dimension ($d_{\text{model}}$), the number of TEM layers, and the window size on \stand's performance across the five datasets, respectively. Overall, the model's performance improves (for almost all metrics) as the model dimension increases. Conversely, performance tends to degrade (for both point-wise and event-level metrics) as the number of TEM layers and the temporal window size increase.

Figures \ref{fig:sen_dmodel1}, \ref{fig:sen_tem1}, and \ref{fig:win_size_all1} also present the impact of $d_{\text{model}}$, the number of TEM layers, and the window size on \stand's performance across the four PSM subsets. Generally, the trend of model performance change is consistent with that observed on the five real-world datasets. Specifically, when the model dimension increases, the performance improves on three subsets (SP2–SP4), while the performance change on SP1 is relatively marginal. Conversely, when the number of TEM layers and the temporal window size increase, performance slightly decreases on the SP2–SP4 subsets, but no clear trend of performance change is observed on SP1.

Therefore, the influence of hyperparameters on \stand~is primarily manifested as follows: When the dataset size is large, the impact is significant, exhibiting a clear performance trend; when the data volume is small, the model is more severely affected by random initialization, leading to less discernible performance trends.

Furthermore, it is important to note that the average level of Aff-F1 and UAff-F1 scores is noticeably better when the training set is SP1 compared to SP2–SP4. This is because these two metrics require the setting of an anomaly evaluation buffer, where predictions within the buffer zone are also regarded as correct. When the anomaly ratio is low, this type of tolerance metric can easily lead to inaccurate evaluations.

% \section{Detailed Visualization Analysis}\label{app:vis}

\ifx\includedfrommain\undefined
    \bibliography{main}
    \end{document}
\fi
